# Supplementary material for: A microstructural rheological model for transient creep in polycrystalline ice
Source: arXiv:2512.08907 ancillary file (2025-12-09)
Supplement: Supplementary file 1 [file Ice_Rheology_Supplemental_Final.pdf]

# *Supplemental Materials*: A microstructural rheological model for transient creep of polycrystalline ice

Alex J. Vargas,[†] Ranjiangshang Ran,[†] and Justin C. Burton[*]

*Department of Physics, Emory University, Atlanta, GA 30322*

## TABLE OF CONTENTS

1 The Rheological Model . . . . . 2
- 1.1 Non-dimensional model . . . . . 2
  - 1.1.1 Dimensional equations . . . . . 2
  - 1.1.2 Dimensionless variables and Π groups . . . . . 2
  - 1.1.3 Reduced form and interpretation . . . . . 3
  - 1.1.4 Nondimensional strain–strain rate behavior . . . . . 3
- 1.2 Prony-series representation of power-law creep . . . . . 5
  - 1.2.1 Log-uniform Prony spectrum . . . . . 5
  - 1.2.2 Proof of the Laplace-Gamma identity . . . . . 7
- 1.3 Dynamics of $c$-axis reorientation in ice grains . . . . . 7

2 Parameter Inference From Experimental Data . . . . . 9
- 2.1 Parameter vector and probabilistic model . . . . . 9
- 2.2 Likelihood function . . . . . 10
- 2.3 Prior and posterior distributions . . . . . 11
- 2.4 Markov chain Monte Carlo sampling . . . . . 11
- 2.5 Autocorrelation and effective sample size . . . . . 12
- 2.6 Gelman–Rubin convergence diagnostic . . . . . 16
- 2.7 Posterior geometry and identifiability . . . . . 17
- 2.8 Prior sensitivity . . . . . 17
- 2.9 Posterior predictive validation . . . . . 17
- References . . . . . 19

Appendix A: Tables and Additional Figures . . . . . 20

---

[†] These authors contributed equally to this work.

[*] Corresponding author: justin.c.burton@emory.edu

# 1. THE RHEOLOGICAL MODEL

## 1.1. Non-dimensional model

Buckingham's Pi theorem states that any physically valid relation among $m$ dimensional variables, expressed in terms of $l$ fundamental units, can be recast in terms of $m - l$ independent dimensionless groups. In our model under constant stress [Eqs. (5) and (6) in the main text], the governing creep laws depend on 7 dimensional variables,

$$\{\varepsilon,\, \dot{\varepsilon},\, t,\, \sigma,\, \beta,\, k,\, \eta_0\},$$

spanning the three base dimensions of mass ($M$), length ($L$), and time ($T$). Thus $m = 7$ and $l = 3$, giving $m - l = 4$ independent dimensionless groups. The parameters $\lambda = \xi_0 \Delta\eta/\eta_0$ and $\sigma/E_0$ are already dimensionless and therefore do not contribute to the count.

### 1.1.1. Dimensional equations

The strain and strain rate under constant applied stress $\sigma$ take the form:

$$\varepsilon(t > 0) = \frac{\sigma}{E_0} + \beta\sigma t^{1/p} + \frac{\sigma\tau_s}{\eta_0} \ln\left(\frac{e^{t/\tau_s} + \lambda}{1 + \lambda}\right), \tag{S1}$$

$$\dot{\varepsilon}(t > 0) = \frac{\beta}{p}\, \sigma t^{(1-p)/p} + \frac{\sigma}{\eta_0(1 + \lambda e^{-t/\tau_s})}, \tag{S2}$$

where $\tau_s = 1/k\sigma^p$ is the microstructural relaxation timescale, $\beta$ and $p$ describe Andrade creep, and $\lambda$ is the dimensionless parameter characterizing the initial viscosity and microstructure.

### 1.1.2. Dimensionless variables and $\Pi$ groups

There are two variables with units of time, $t$ and $1/\dot{\varepsilon}$, and three independent timescales, $\tau_s$, $1/(\beta\sigma)^p$, and $\eta_0/\sigma$. The last timescale is really an inverse shear rate. We form 4 dimensionless groups by normalizing by $\tau_s$:

$$\Pi_1 = \tilde{t} \equiv \frac{t}{\tau_s}, \tag{S3a}$$

$$\Pi_2 = \tilde{\dot{\varepsilon}} \equiv \dot{\varepsilon}\tau_s, \tag{S3b}$$

$$\Pi_3 = C \equiv \beta\sigma\tau_s^{1/p}, \tag{S3c}$$

$$\Pi_4 = D \equiv \frac{\sigma\tau_s}{\eta_0}, \tag{S3d}$$

Together with $\lambda$ and $\sigma/E_0$, these dimensionless ratios fully characterize the response. Physically, $C$ sets the magnitude of the Andrade power-law creep, $D$ sets the infinite-time effective viscosity, $\lambda$ controls the initial microstructural viscosity, and $\sigma/E_0$ is the initial jump in strain due to the Young's modulus of ice.

### 1.1.3. Reduced form and interpretation

Rewriting Eqs. (S1)–(S2) in terms of the dimensionless groups yields:

$$\varepsilon(\tilde{t} > 0) = \frac{\sigma}{E_0} + C\,\tilde{t}^{1/p} + D\,\ln\left(\frac{e^{\tilde{t}} + \lambda}{1 + \lambda}\right), \tag{S4}$$

$$\tilde{\dot{\varepsilon}}(\tilde{t} > 0) = \frac{C}{p}\,\tilde{t}^{(1-p)/p} + \frac{D}{1 + \lambda e^{-\tilde{t}}}. \tag{S5}$$

In this dimensionless form, the primary Andrade creep response is set by $C$ and $p$. The tertiary regime is set by a plateau at $\tilde{\dot{\varepsilon}} = D$. Eqs. S4-S5 cannot be solved analytically for $\tilde{\dot{\varepsilon}}$ as a function of $\varepsilon$, nor is there an analytical expression for the position of $\tilde{\dot{\varepsilon}}_{\min}$. However, they represent a compact mathematical expression to describe the transient behavior observed in ice rheology experiments under constant stress.

### 1.1.4. Nondimensional strain–strain rate behavior

Figure S1 shows the strain–strain rate curves in the nondimensional form of Eqs. (S4)–(S5). For the Treverrow *et al.* [1] (2012) tests in panel (a), all four experiments share the same Andrade exponent $p$, so their primary branches have identical slopes. The relevant question is whether the magnitudes of $\tilde{\dot{\varepsilon}} = \dot{\varepsilon}\tau_s$ align. At each stress level the isotropic and anisotropic curves lie reasonably close together in the primary regime, which is consistent with similar values of $C$ at fixed $\sigma_0$. The curves separate near the strain rate minimum, as expected, because the location and depth of the minimum depend sensitively on the softening parameter $\lambda$, and the inferred $\lambda$ values differ between samples.

In the tertiary regime the curves do not collapse onto a single plateau. Both 0.2 MPa tests approach similar long-time values of $\tilde{\dot{\varepsilon}}$, the isotropic 0.4 MPa test approaches a higher value, and the anisotropic 0.4 MPa test remains below the other three curves. This pattern reflects the combined effect of changes in the relaxation time $\tau_s = (k\sigma_0^p)^{-1}$ and in the structural coefficient $D$, both of which are set by the inferred structural parameters $k$ and $A_0$. The nondimensional curves show that differences in the long-time response are dominated by the stress-dependence

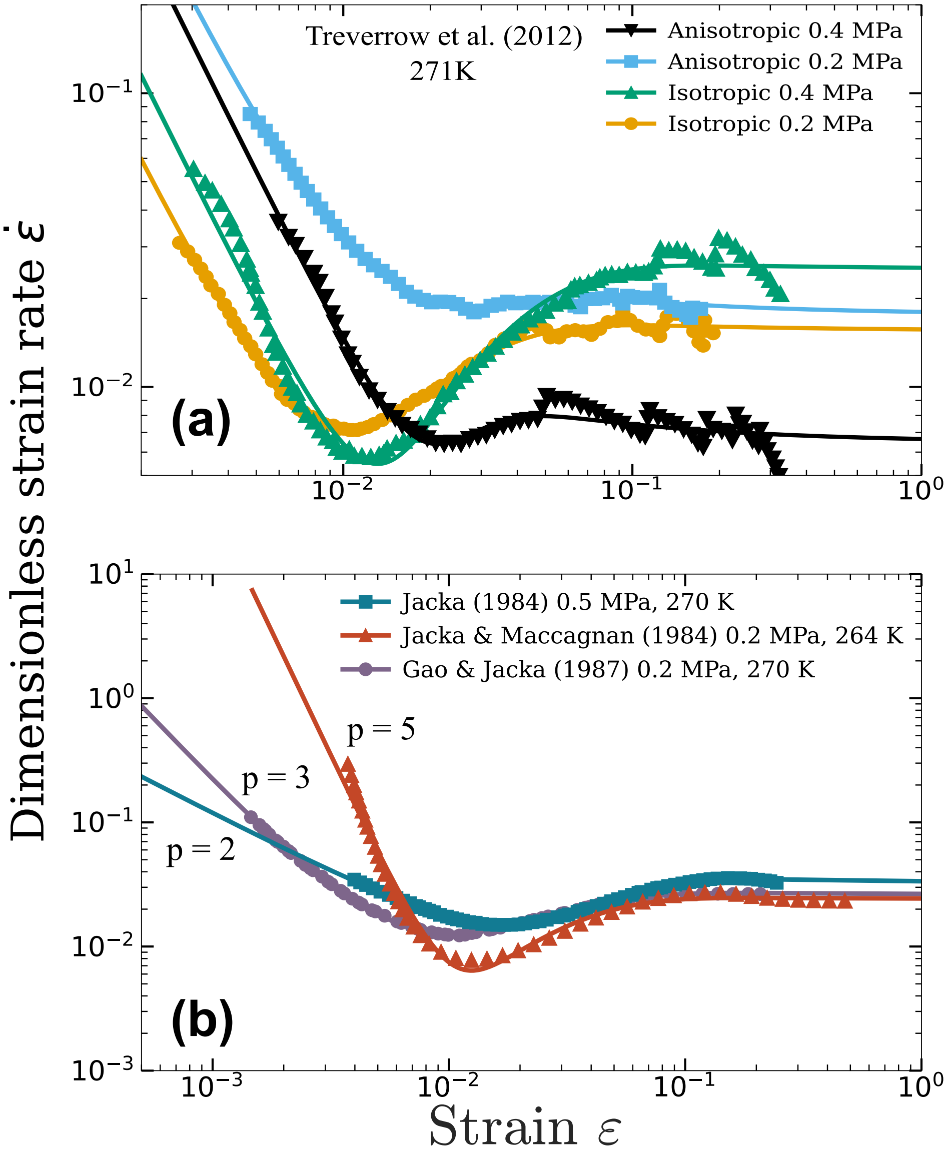


FIG. S1. Nondimensional strain–strain rate curves from Eqs. (S4)–(S5). (a) Treverrow *et al.* [1] (2012) tests at 271 K. The primary Andrade branches align at fixed stress, the minima differ due to variations in $\lambda$, and the tertiary values group by stress, with the anisotropic 0.4 MPa curve lying below the others. (b) Additional datasets from Jacka [2] (1984), Jacka and Maccagnan [3] (1984), and Gao and Jacka [4] (1987). These experiments have different $p$ values, so only the tertiary regime is directly comparable; its grouping by stress and temperature is consistent with the behavior in panel (a).

of the structural relaxation rate ($k$) and softening strength ($\lambda$), rather than by initial fabric (isotropic vs. anisotropic) alone.

Panel (b) shows three additional datasets, from Jacka [2] (1984), Jacka and Maccagnan [3]

(1984), and Gao and Jacka [4] (1987). These experiments were performed at different temperatures and stresses and are fit with different Andrade exponents $p$, so a detailed comparison of the primary regime is not meaningful. However, the tertiary portions of the nondimensional curves approach similar values of $\tilde{\dot{\varepsilon}}$ when grouped by stress and temperature, despite the differing $p$. This supports the view that the model captures a common structure for the long-time creep response while the remaining differences between curves reflect genuine variation in the underlying structural relaxation parameters.

## 1.2. Prony-series representation of power-law creep

### 1.2.1. Log-uniform Prony spectrum

We can construct a power-law (Andrade) creep, $\varepsilon \propto t^{1/p}$, from a number $N$ of Kelvin–Voigt elements connected in series. Under a heaviside step stress, $\sigma$, the strain of a single element in the series is:

$$\varepsilon_i(t) = \frac{\sigma}{E_i}\big(1 - e^{-t/\tau_i}\big), \qquad \tau_i = \frac{\eta_i}{E_i}. \tag{S6}$$

The total strain corresponds to a Prony-series representation [5]:

$$\varepsilon(t) = \sum_{i=1}^{N} \frac{\sigma}{E_i}\big(1 - e^{-t/\tau_i}\big). \tag{S7}$$

For each Kelvin-Voigt element, we assign a distinct timescale $\tau_i$, which is constructed to be uniformly and logarithmically spaced in $[\tau_{\min}, \tau_{\max}]$:

$$\tau_i = \tau_{\min} r^{i-1}, \qquad \tau_{\max} = \tau_N = \tau_{\min} r^{N-1}, \tag{S8}$$

where $r = \tau_{i+1}/\tau_i > 1$ is a ratio of timescales. Note that the spacing for $\ln \tau$ is a constant:

$$\Delta = \Delta \ln \tau = \ln \tau_{i+1} - \ln \tau_i = \ln r. \tag{S9}$$

This allows us to construct a Riemann sum by inserting $(\Delta/\Delta)$ to Eq. (S7):

$$\varepsilon(t) = \sum_{i=1}^{N} \frac{\sigma}{E_i \Delta}\big(1 - e^{-t/\tau_i}\big)\Delta. \tag{S10}$$

In the limits of $r \to 1$ and $\Delta \to 0$, the Riemann sum becomes a Riemann integral for the variable $\ln \tau$:

$$\varepsilon(t) = \lim_{\Delta \to 0} \sum_{i=1}^{N} \frac{\sigma}{E_i \Delta}\big(1 - e^{-t/\tau_i}\big)\Delta = \int_{\ln \tau_{\min}}^{\ln \tau_{\max}} \frac{\sigma}{E(\tau)}\left(1 - e^{-t/\tau}\right) d(\ln \tau) \tag{S11}$$

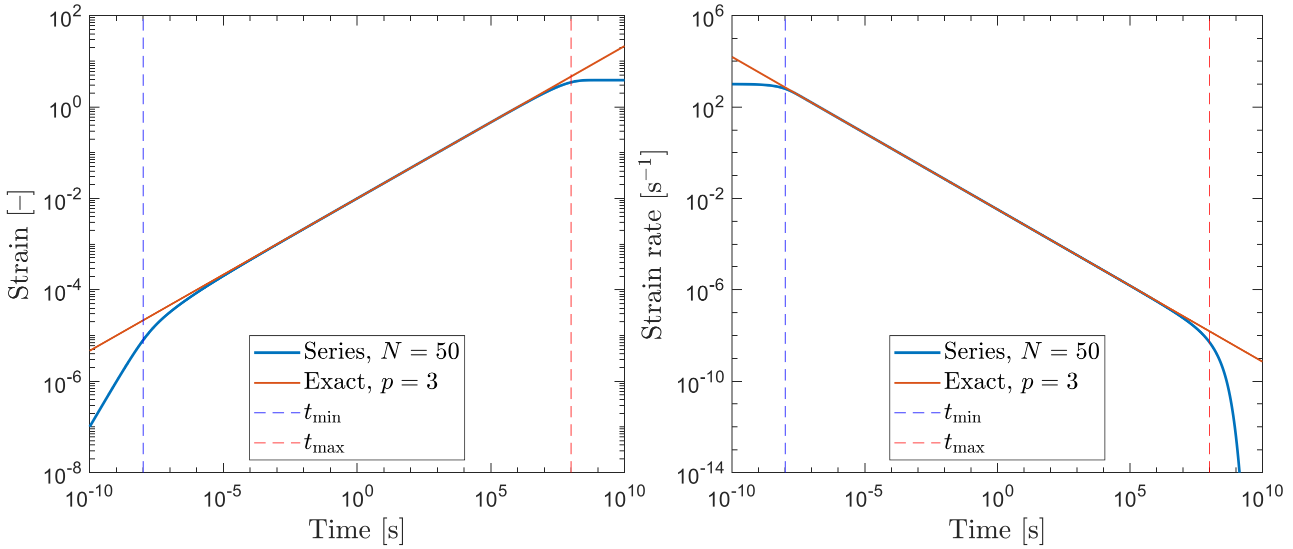


FIG. S2. Power-law creep approximated by a series of Kelvin-Voigt elements with $N = 50$. Left: the exact and approximated strain for power-law creep, $\varepsilon \propto t^{1/p}$; right: the exact and approximated strain rate, $\dot{\varepsilon} \propto t^{1/p-1}$, with the exponent $p = 3$. The discrete series approximate the exact power law well within the time interval $[\tau_{\min}, \tau_{\max}]$. Here, $\tau_{\min} = 10^{-8}$ s and $\tau_{\max} = 10^{8}$ s.

$$= \int_{\tau_{\min}}^{\tau_{\max}} \frac{\sigma}{\tau E(\tau)} \left(1 - e^{-t/\tau}\right) d\tau. \tag{S12}$$

Note that the following Laplace-Gamma identity holds for $p > 1$, which is proved later in this document:

$$t^{1/p} = \frac{-1}{\Gamma(-1/p)} \int_0^{\infty} \left(1 - e^{-t/\tau}\right) \tau^{\frac{1}{p}-1}\, d\tau, \tag{S13}$$

where $\Gamma(x)$ is the Gamma function. By comparing Eqs. (S12) and (S13) in the limits of $\tau_{\min} \to 0$ and $\tau_{\max} \to \infty$, one would find that the strain converges to the desired power-law form, $\epsilon = \beta\sigma t^{1/p}$, given the following $E(\tau)$:

$$E(\tau) = -\frac{\Gamma(-1/p)}{\beta\tau^{1/p}} = \Gamma\left(1 - \frac{1}{p}\right) \frac{p}{\beta\tau^{1/p}}. \tag{S14}$$

The continuous spectrum $E(\tau)$ can be approximated by the discrete form $E_i(\tau_i)$:

$$E_i(\tau_i) = \Gamma\left(1 - \frac{1}{p}\right) \frac{p}{\beta\tau_i^{1/p}\Delta} = \Gamma\left(1 - \frac{1}{p}\right) \frac{p}{\beta\tau_i^{1/p}\ln r}. \tag{S15}$$

Figure S2 shows the strain and strain rate of a power-law creep of $p = 3$, approximated by a discrete series of $N = 50$ Kelvin Voigt elements, whose elastic moduli $E_i$ are set by Eq. (S15). The discrete approximation works well within the time interval of $[\tau_{\min}, \tau_{\max}]$, where we set $\tau_{\min} = 10^{-8}$ s and $\tau_{\max} = 10^{8}$ s.

### 1.2.2. Proof of the Laplace-Gamma identity

The Laplace-Gamma identity in Eq. (S13) can be proved as follows. Start with the inverse Laplace transform of a power-law function, which holds for $\mathrm{Re}(\alpha) > 0$:

$$t^{-\alpha} = \frac{1}{\Gamma(\alpha)} \int_0^\infty s^{\alpha-1} e^{-st} ds. \tag{S16}$$

Subtract two inverse Laplace transforms of different transform variables to get:

$$q^{-\alpha} - t^{-\alpha} = \frac{1}{\Gamma(\alpha)} \int_0^\infty s^{\alpha-1} (e^{-sq} - e^{-st}) ds. \tag{S17}$$

Set $\alpha = -\mu$ with $0 < \mu < 1$ and $q \to 0^+$. Although the integral in Eq. (S16) diverges when $\mathrm{Re}(\alpha) < 0$, the difference between the two inverse Laplace transform in Eq. (S17) converge by analytic continuation, which leads to:

$$\lim_{q \to 0^+} (q^\mu - t^\mu) = \frac{1}{\Gamma(-\mu)} \int_0^\infty s^{-\mu-1} (1 - e^{-st}) ds. \tag{S18}$$

This shows that the following identity is true for $0 < \mu < 1$:

$$t^\mu = \frac{-1}{\Gamma(-\mu)} \int_0^\infty \left(1 - e^{-st}\right) s^{-\mu-1} ds. \tag{S19}$$

Apply a change of variables, $s = 1/\tau$, such that $ds = -\tau^{-2} d\tau$, and we get:

$$t^\mu = \frac{-1}{\Gamma(-\mu)} \int_0^\infty \left(1 - e^{-t/\tau}\right) \tau^{\mu-1} d\tau. \tag{S20}$$

Replace $\mu$ with $1/p$, with $p > 1$, and we arrive at the Laplace-Gamma identity:

$$t^{1/p} = \frac{-1}{\Gamma(-1/p)} \int_0^\infty \left(1 - e^{-t/\tau}\right) \tau^{\frac{1}{p}-1} d\tau. \tag{S21}$$

## 1.3. Dynamics of $c$-axis reorientation in ice grains

Plastic deformation of polycrystalline ice occurs predominantly by basal slip, an anisotropic mechanism that both shears the crystal lattice and induces a plastic spin[6–8]. The resulting lattice rotation is described kinematically by:

$$\dot{\mathbf{R}}\mathbf{R}^{-1} = \mathbf{W}^p, \tag{S22}$$

where $\mathbf{R}$ is the lattice rotation tensor and $\mathbf{W}^p$ is the plastic spin generated by slip on the active crystallographic systems. Each grain therefore rotates in orientation space as it deforms, and an initially random polycrystal progressively develops a preferred orientation (fabric)[9, 10]. In

a continuum description, the evolution of a grain's $c$-axis orientation vector $\mathbf{c}$ can be written in the standard crystal-plasticity form:

$$\frac{d\mathbf{c}}{dt} = \mathbf{W}^g \cdot \mathbf{c} + \lambda \left( \mathbf{D}^g \cdot \mathbf{c} - \left( \mathbf{c} \cdot \mathbf{D}^g \cdot \mathbf{c} \right) \mathbf{c} \right), \tag{S23}$$

where $\mathbf{D}^g$ and $\mathbf{W}^g$ are the grain-level strain-rate and spin tensors, and $\lambda = O(1)$ is a geometric factor. Because basal slip dominates in ice, the $\mathbf{D}^g$ term governs the rotation: grains with misoriented $c$-axes rotate toward the compressive stress axis, producing the familiar alignment seen in laboratory fabrics. The orientation distribution function (ODF) of the aggregate is therefore advected in orientation space by the rotation velocity (S23), sharpening over a finite strain interval as grains migrate toward stable orientations.

Under uniaxial compression with strain rate $\dot{\varepsilon}$, the macroscopic strain rate tensor is:

$$\mathbf{D} = \dot{\varepsilon} \begin{pmatrix} -1/2 & 0 & 0 \\ 0 & -1/2 & 0 \\ 0 & 0 & 1 \end{pmatrix},$$

and restricting $\mathbf{c}$ to the $xz$-plane with $\mathbf{c} = (\sin\theta, 0, \cos\theta)$, Eq. (S23) reduces to:

$$\dot{\theta} = \frac{\lambda \dot{\varepsilon}}{2} \sin(2\theta). \tag{S24}$$

This expression captures the essential geometry: grains rotate fastest when $\theta \approx 45^\circ$ and slow as they align with the compressive axis. Integrating (S24) gives the characteristic alignment timescale:

$$\tau_{\text{align}} = \frac{1}{\lambda \dot{\varepsilon}} \ln\left( \frac{\tan\theta_0}{\tan\theta_f} \right), \tag{S25}$$

showing that lattice alignment proceeds on a time inversely proportional to the strain rate. If slip obeys a stress-dependent power law $\dot{\varepsilon} \propto \sigma^n$[11], then:

$$\tau_{\text{align}}(\sigma) \propto \sigma^{-n}. \tag{S26}$$

Our model used in the main text prescribes an internal viscosity of the form:

$$\eta(t) = \eta_0 + \Delta\eta e^{-t/\tau_s(\sigma)},$$

where $\tau_s(\sigma)$ controls microstructural rearrangement. Equations (S24)–(S26) show that grain rotation under deviatoric stress possesses an intrinsic relaxation time with the same stress dependence as $\tau_s(\sigma)$, suggesting a natural micromechanical interpretation: the structured dashpot encodes the rate at which an initially isotropic fabric evolves towards an aligned, lower-viscosity state through slip-driven lattice rotation. Empirically, we choose $n$ to be the same as the Andrade exponent $p$ such that the strain at the minimum is $\varepsilon_{\text{min}} \approx 1\%$.

# 2. PARAMETER INFERENCE FROM EXPERIMENTAL DATA

To infer the physical parameters appearing in Eqs. (S1) and (S2), we perform Bayesian inference using Markov chain Monte Carlo (MCMC) sampling. The following sections present the full probabilistic formulation of the inference problem, including the likelihood in log-space, the specification of broad lognormal priors, and the ensemble-based sampling strategy employed in `emcee` [12]. Our implementation utilizes a mixture of affine-invariant ensemble moves (DEMove, DESnookerMove, and the stretch move), with an adaptive KDE proposal added during production sampling to improve exploration of correlated directions. We additionally describe the automatic rejection of invalid parameter proposals, burn-in and sampler reset, outlier-walker filtering, and multiple convergence diagnostics, including integrated autocorrelation times, effective sample sizes, Gelman–Rubin statistics, and the bulk/tail $\hat{R}$ measures from ArviZ. The overall methodology follows the general Bayesian framework used for nonlinear viscoelastic inference in Ran *et al.* [13, 14], extended here to recover the parameters governing the full transient response of our model.

## 2.1. Parameter vector and probabilistic model

The inference problem is formulated in terms of a five dimensional parameter vector,

$$\theta = \{\log_{10} B,\ \log_{10} k,\ \log_{10} A_0,\ \log_{10} \lambda,\ \log_{10} \sigma_{\text{noise}}\}, \tag{S27}$$

where each physical parameter is expressed in log-space to ensure positivity and to enable efficient exploration over the several-decade dynamic ranges characteristic of ice creep rheology. The parameter $\sigma_{\text{noise}}$ represents the effective observational noise level in $\log_{10}$–strain-rate space and absorbs both experimental measurement variability and small model–data mismatches across the full transient creep response.

Given an experimental dataset,

$$D = \{\varepsilon_i,\ \dot{\varepsilon}_i^{\text{obs}}\},$$

collected at fixed applied stress $\sigma_0$, we seek the posterior distribution,

$$P(\theta \mid D) = \frac{P(D \mid \theta)\, P(\theta)}{\displaystyle\int P(D \mid \theta')\, P(\theta')\, d\theta'}, \tag{S28}$$

where the denominator is the Bayesian evidence, included for completeness but not needed for

parameter estimation. This formulation yields the joint distribution of all model parameters consistent with the observed transient creep curves.

### 2.2. Likelihood function

Evaluating the posterior distribution in Eq. (S28) requires specifying the statistical relationship between our model and the experimental observations. We therefore define the likelihood function $P(D \mid \theta)$, which measures the discrepancy between predicted and observed strain rates. Because the experimental creep curves span several decades in $\dot{\varepsilon}$, the misfit is evaluated in $\log_{10}$-space. We define:

$$y_i = \log_{10} \dot{\varepsilon}_i^{\text{obs}}, \qquad f_i(\theta) = \log_{10} \dot{\varepsilon}^{\text{model}}(t_i; \theta),$$

where $\dot{\varepsilon}^{\text{model}}(t)$ is computed from Eq. (S2) and interpolated onto the experimental data points. Model predictions are interpolated using a shape-preserving PCHIP interpolant, which avoids spline overshoot and ensures numerically stable evaluation at the experimental sampling points, even when the strain-rate curve is non-monotonic. The observational model is:

$$y_i = f_i(\theta) + \eta_i, \qquad \eta_i \sim \mathcal{N}(0, \sigma_{\text{noise}}^2), \tag{S29}$$

which assumes independent Gaussian fluctuations in log-space.

This leads to the likelihood,

$$P(D \mid \theta) = (2\pi\sigma_{\text{noise}}^2)^{-N/2} \exp\left[ -\frac{1}{2\sigma_{\text{noise}}^2} \sum_{i=1}^{N} (y_i - f_i(\theta))^2 \right], \tag{S30}$$

and the corresponding log-likelihood,

$$L(D \mid \theta) = \ln P(D \mid \theta) = -\frac{N}{2} \ln(2\pi\sigma_{\text{noise}}^2) - \frac{1}{2\sigma_{\text{noise}}^2} \sum_{i=1}^{N} (y_i - f_i(\theta))^2. \tag{S31}$$

During sampling, any parameter proposals that produce invalid or nonphysical model predictions—such as non-monotonic strain, non-positive strain rates, NaNs/Infs, or interpolation failures—is automatically assigned $L = -\infty$ and rejected. This ensures numerical stability across the full parameter space.

### 2.3. Prior and posterior distributions

Each free parameter is assigned a lognormal prior by placing a Gaussian prior in log-space:

$$P(\theta) = \prod_{j=1}^{5} \frac{1}{\sqrt{2\pi}\sigma_j} \exp\left[-\frac{(\theta_j - \mu_j)^2}{2\sigma_j^2}\right], \qquad \sigma_j = 3.0, \tag{S32}$$

corresponding to a three-decade uncertainty for all parameters. Dataset-specific prior means $\mu_j$ are listed in Tables S1–S2 in *Tables and Additional Figures.* These broad priors regularize the nonlinear inversion while allowing the sampler to explore physically plausible ranges without drifting into pathological regions where Eq. S2 becomes numerically unstable or undefined. Combining Eqs. (S30) and (S32), the unnormalized posterior distribution is:

$$P(\theta \mid D) \propto \exp\left[-\frac{1}{2\sigma_{\text{noise}}^2} \sum_{i=1}^{N} (y_i - f_i(\theta))^2\right] \times \exp\left[-\sum_{j=1}^{5} \frac{(\theta_j - \mu_j)^2}{2\sigma_j^2}\right]. \tag{S33}$$

### 2.4. Markov chain Monte Carlo sampling

Posterior exploration is performed using the affine-invariant ensemble sampler implemented in `emcee` [12], which generalizes the classical Metropolis–Hastings framework. Although the Metropolis–Hastings formulation may be expressed in terms of Gaussian perturbations,

$$\theta' = \theta + \delta, \qquad \delta \sim \mathcal{N}(0, \Sigma), \tag{S34}$$

with the acceptance ratio,

$$\alpha = \min\left[1, \frac{P(D \mid \theta')P(\theta')}{P(D \mid \theta)P(\theta)}\right]. \tag{S35}$$

In practice the sampler operates using a mixture of ensemble updates that improve sampling efficiency for correlated or anisotropic posteriors.

A substantial fraction of proposals are generated by the affine-invariant stretch move. For a walker $k$ and a randomly chosen partner $j \neq k$, the proposal is:

$$\theta'_k = \theta_j + z(\theta_k - \theta_j), \tag{S36}$$

where the stretch factor $z$ is drawn from:

$$g(z) \propto z^{-1/2}, \qquad z \in [1/a,\, a], \tag{S37}$$

with $a = 2$. The corresponding acceptance probability is:

$$\alpha = \min\left[1,\ z^{d-1}\frac{P(D \mid \theta'_k)P(\theta'_k)}{P(D \mid \theta_k)P(\theta_k)}\right], \tag{S38}$$

where $d = 5$ is the dimensionality of the parameter vector. In addition to the stretch move, `emcee`'s production stage uses a fixed mixture of DEMove, DESnookerMove, and an adaptive KDEMove, which together improve exploration of weakly identified directions associated with the full transient curve.

Initial walker positions are drawn from Gaussian balls centered on the prior means with widths equal to the prior standard deviation. For each experimental dataset, we evolve an ensemble of $N_{\text{walkers}} = 64$ walkers for 25,000 iterations. The first 10,000 iterations are discarded as burn-in, leaving a stationary ensemble of posterior samples. A small number of walkers nevertheless drift into persistently low probability regions of parameter space, typically becoming trapped in shallow local minima or exploring flat directions far from the main posterior mode. These walkers are identified using a $3\sigma$ cutoff applied to the per-walker mean log-likelihood and removed prior to flattening the chains.

To illustrate typical sampler performance, we present diagnostic plots for one representative dataset (Treverrow *et al.* [1], 0.2 MPa). Figure S3 presents the prior-to-posterior distributions, demonstrating how the data constrain each parameter relative to the broad, three-decade priors. Figure S4 shows the corresponding trace plots, which indicate rapid mixing, clean post–burn-in stationarity, and the absence of long-lived metastable states. The pairwise correlation structure of the posterior is shown in Figure S5, highlighting anisotropic but unimodal geometry in the $(k, \lambda)$ subspace and tight constraints on $(B, A_0)$.

Together, these diagnostics provide a concise summary of sampler performance, parameter identifiability, and posterior structure. Complete diagnostic figures for all datasets— including trace plots, correlation matrices, and prior–posterior histograms—are provided in *Tables and Additional Figures*.

### 2.5. Autocorrelation and effective sample size

Chain quality is quantified through the integrated autocorrelation time,

$$\tau_{\text{int}} = \frac{1}{2} + \sum_{t=1}^{\infty} \rho(t), \tag{S39}$$

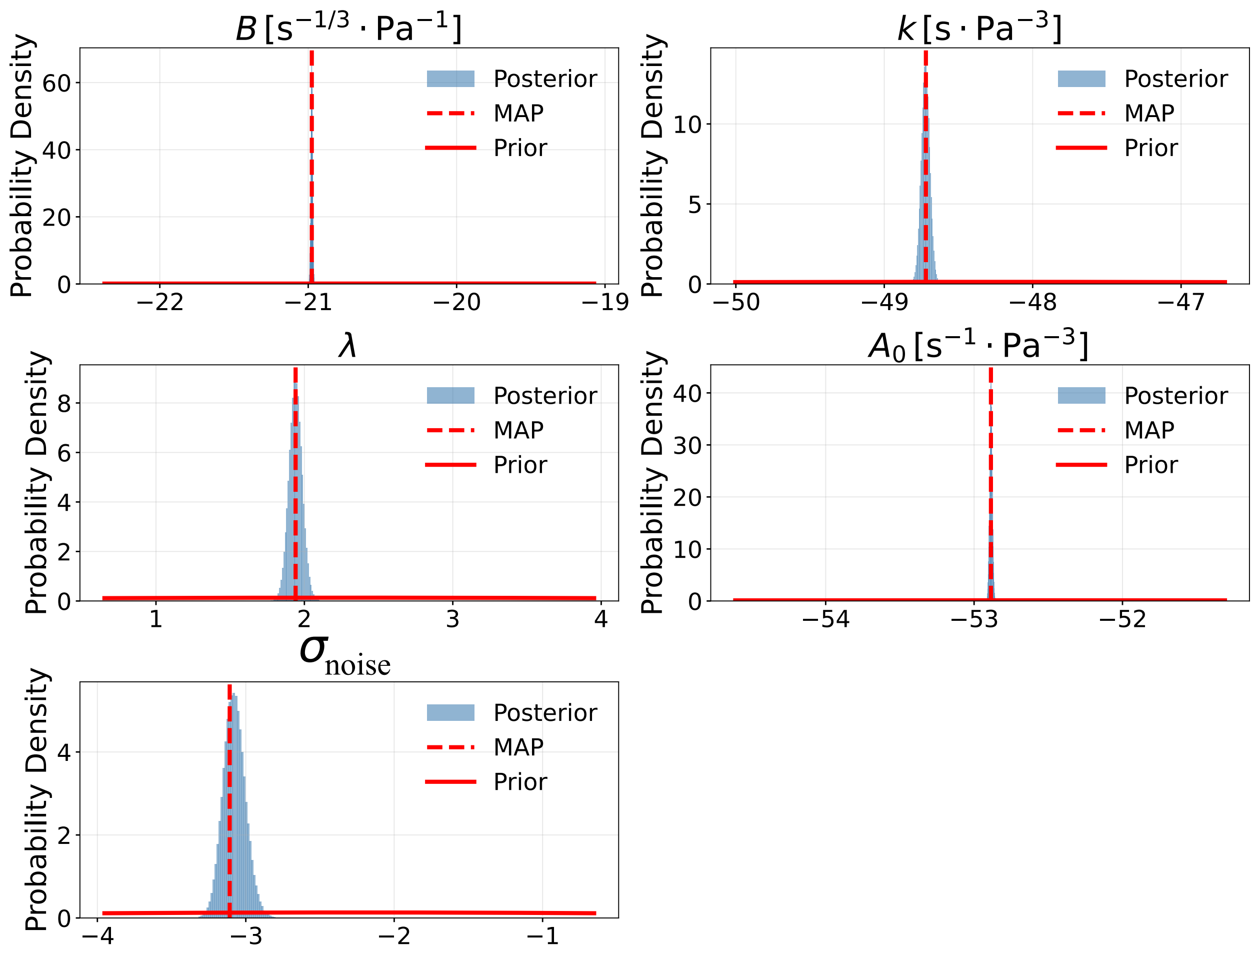


FIG. S3. Prior-to-posterior comparison for the isotropic .2 MPa experiment from Treverrow *et al.* [1]. The data strongly constrain $B$ and $A_0$, while $k$ and $\lambda$ exhibit broader posteriors, consistent with their roles in shaping the transient relaxation behavior. Full histograms for all datasets appear in the *Appendix A: Tables and Additional Figures*

where $\rho(t)$ denotes the normalized autocorrelation at lag $t$. Across the full suite of datasets, the autocorrelation times were consistently small,

$$\tau_{\mathrm{int}} \approx 20\text{--}40,$$

with the lower end corresponding to well-constrained parameters (e.g. $B$ and $A_0$) and the upper end associated with comparatively shallow posterior directions (e.g. $k$ and $\lambda$). The corresponding effective number of independent samples is:

$$N_{\mathrm{eff}} = \frac{N_{\mathrm{walkers}}\,N_{\mathrm{steps}}}{2\tau_{\mathrm{int}}}. \tag{S40}$$

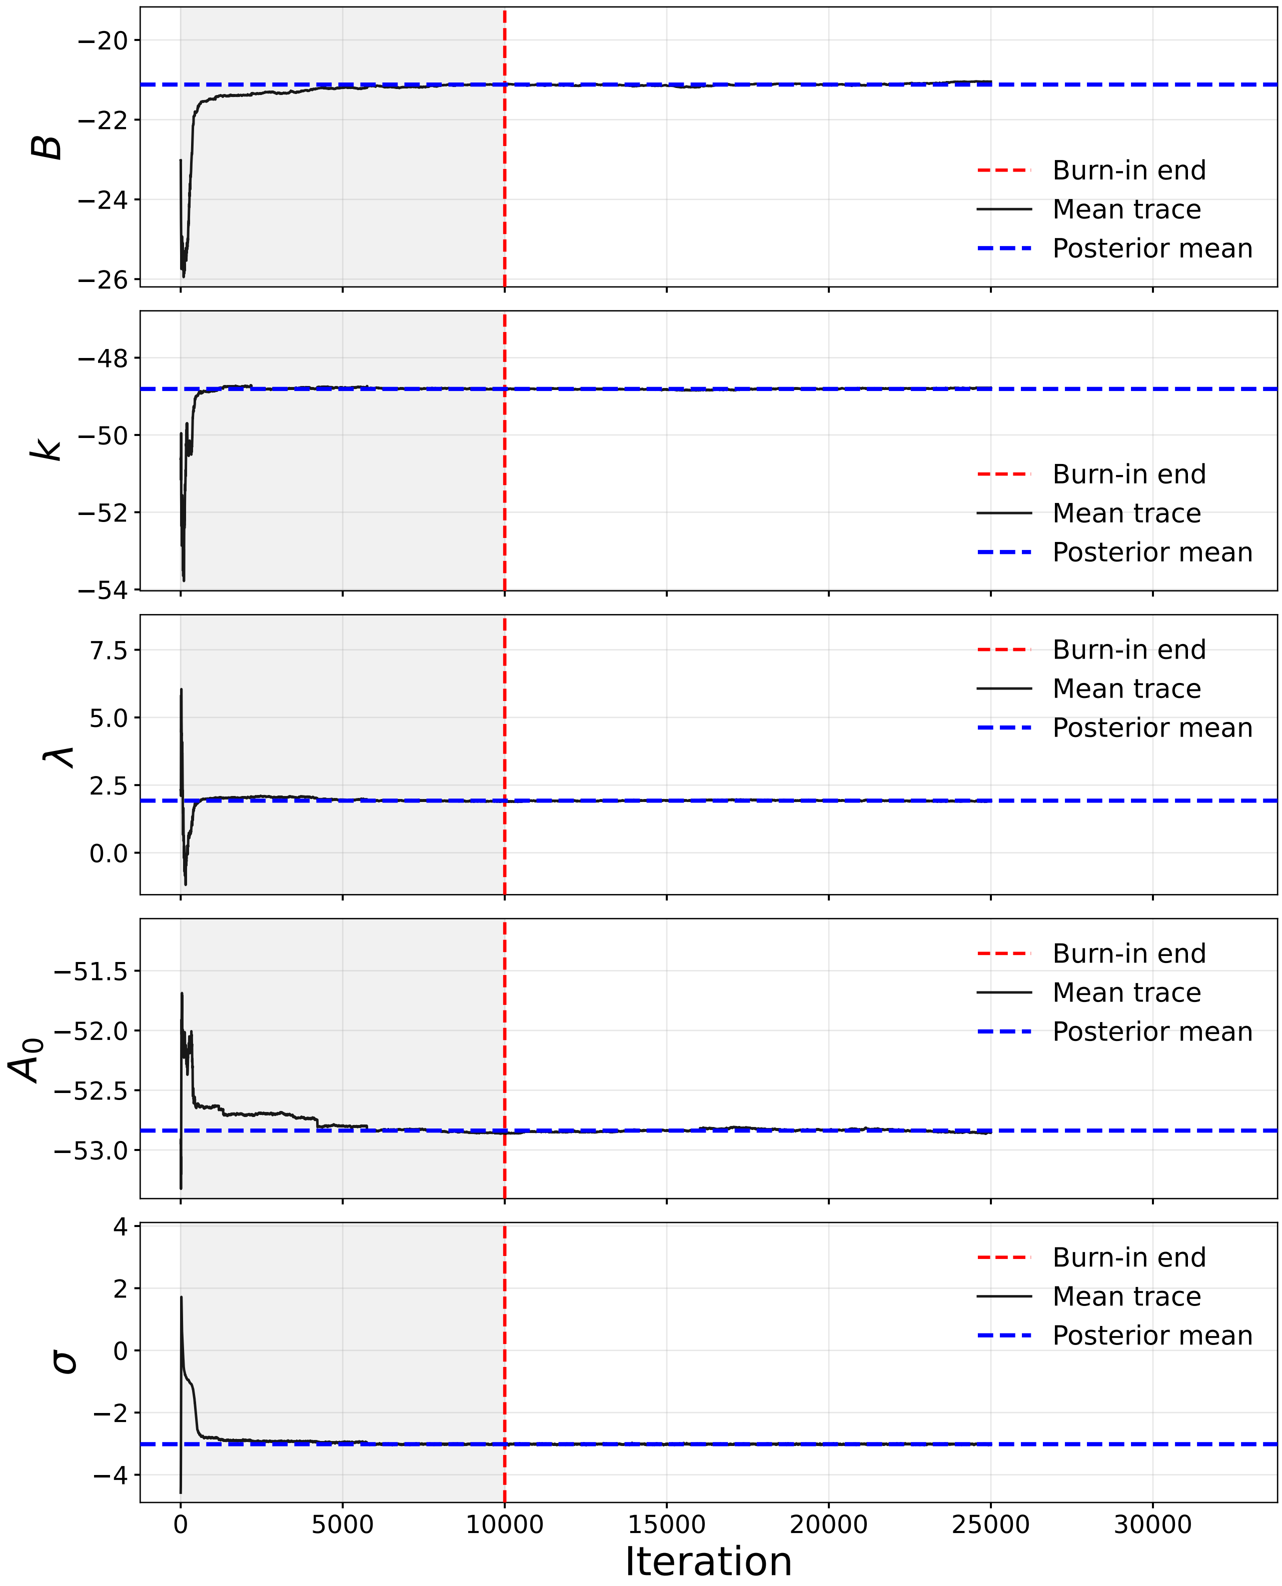


FIG. S4. Representative trace plots for the isotropic .2 MPa experiment from Treverrow *et al.* [1].The chains mix rapidly and show no evidence of metastable states or slow drifts.

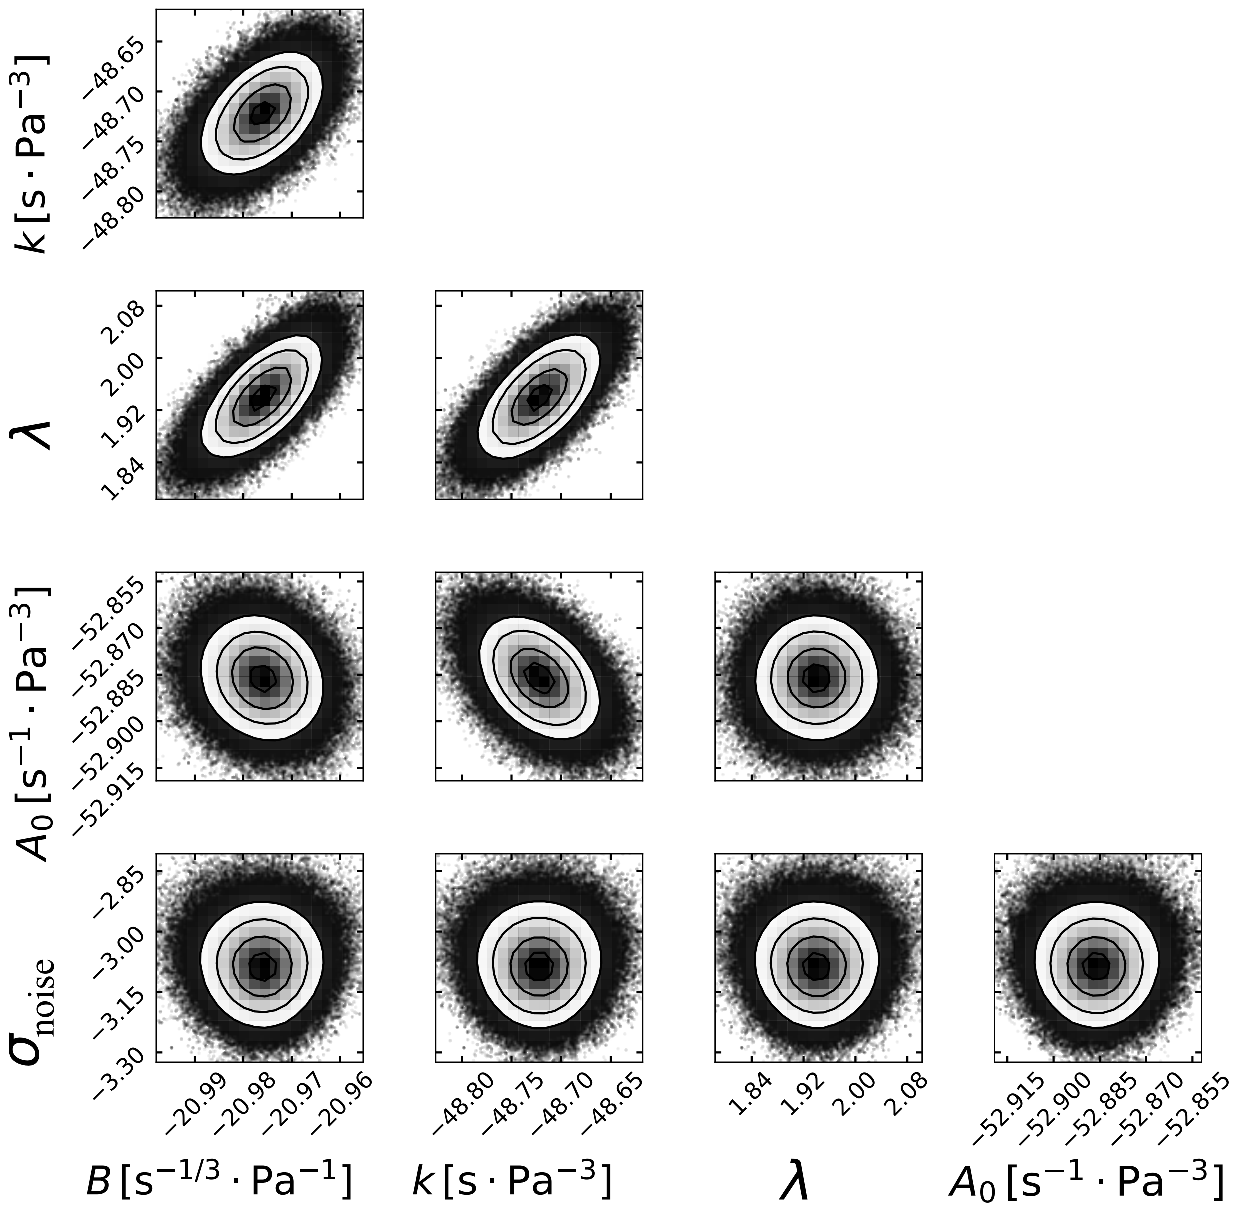


FIG. S5. Pairwise parameter correlations for the isotropic .2 MPa experiment from Treverrow *et al.* [1] based on flattened post–burn-in samples. The posterior displays modest elongation in the $(k, \lambda)$ plane but remains unimodal and well-localized.

All chains show strong convergence diagnostics. The Treverrow *et al.* [1] (2012) and Jacka and Maccagnan [3] (1984) fits achieve large effective sample sizes, $N_{\text{eff}} \sim 2 \times 10^4$–$5 \times 10^4$, while Gao and Jacka [4] (1987) yields $N_{\text{eff}} \approx 10^3$. These values are well above common guidelines

($N_{\text{eff}} \gtrsim 100$), indicating excellent chain mixing and sufficient independent information for stable posterior estimation.

In all runs, the sampler is explicitly reset after the burn-in phase, so the production chain consists solely of samples drawn from the stationary distribution. The full chains (burn-in and production) are retained for diagnostic plots but only production samples are used for posterior statistics.

### 2.6. Gelman–Rubin convergence diagnostic

To assess convergence across the ensemble, we compute the Gelman–Rubin potential scale reduction factor $\hat{R}$ for each parameter. For $M$ chains of length $N$, let $\bar{\theta}_m$ denote the mean of chain $m$ and $\bar{\theta}$ the mean across chains.

*Between-chain variance:*

$$B = \frac{N}{M-1} \sum_{m=1}^{M} (\bar{\theta}_m - \bar{\theta})^2. \tag{S41}$$

*Within-chain variance:*

$$W = \frac{1}{M} \sum_{m=1}^{M} s_m^2, \qquad s_m^2 = \frac{1}{N-1} \sum_{i=1}^{N} (\theta_{m,i} - \bar{\theta}_m)^2. \tag{S42}$$

*Marginal posterior variance estimate:*

$$\hat{V} = \frac{N-1}{N} W + \frac{1}{N} B. \tag{S43}$$

*Gelman–Rubin statistic:*

$$\hat{R} = \sqrt{\frac{\hat{V}}{W}}. \tag{S44}$$

Values of $\hat{R}$ close to 1 indicate that the chains have mixed to the same stationary distribution. Across all datasets, we obtain:

$$\hat{R} = 1.00\text{–}1.09,$$

comfortably within the conventional convergence threshold ($\hat{R} < 1.1$). No systematic inflation of $\hat{R}$ was observed in the parameters or datasets, and slightly higher values occurred in parameters associated with flatter posterior directions.

For completeness, we also compute the bulk and tail $\hat{R}$ diagnostics using the ArviZ package. Both statistics remain below 1.1 for all parameters, providing independent confirmation that the chains exhibit no signs of nonstationarity, long-lived transients, or undetected metastability.

### 2.7. Posterior geometry and identifiability

To quantify dependencies between parameters, we compute the Pearson correlation coefficient,

$$\rho(X, Y) = \frac{\mathrm{cov}(X, Y)}{\sigma_X \sigma_Y}, \tag{S45}$$

using the flattened post-burn-in samples. The corner plots (Figs. S5, S20–S25) reveal elongated joint distributions, particularly in the $(k, \lambda)$ plane. These correlations arise from the coupled influence of $k$ and $\lambda$ on the transient relaxation dynamics of the our model, which produces shallow ridges rather than discrete modes in the likelihood surface.

Moderate correlation is also observed between $(B, A_0)$, reflecting their partially compensatory roles in controlling the early-time Andrade decay and the late-time viscous response. Aside from these physically interpretable anisotropies, the posterior distributions show no evidence of multimodality or isolated secondary maxima. Across all datasets, the joint posterior landscape is smooth and unimodal, with only modest elongation along the $(k, \lambda)$ directions and no indication of competing modes or disconnected regions of high probability. This global structure is fully consistent with the excellent mixing of the sampler, the short integrated autocorrelation times, and the near-unity Gelman–Rubin $\hat{R}$ values reported above.

### 2.8. Prior sensitivity

To verify robustness with respect to the chosen priors, we repeat selected MCMC fits with prior means shifted by $\pm 1$ decade in each parameter. The resulting posterior means shift by no more than 5%, and posterior widths remain nearly unchanged, indicating that the data, rather than the priors, primarily determine the inferred parameters. This prior-insensitivity further supports the identifiability of the Andrade and microstructured-dashpot contributions over the parameter range probed by the experiments.

### 2.9. Posterior predictive validation

The model reproduces the full transient evolution $\dot{\varepsilon}(t)$ across all datasets, including the Andrade-like primary creep regime, the strain-rate minimum, and the late-time viscous asymptote. The posterior-predictive bands encompass the observed curves with deviations well within the inferred observational noise scale $\sigma_{\text{noise}}$, confirming both the adequacy of the model and the consistency of the inferred parameters. No systematic deviations were observed, and the posterior predictive envelopes showed no evidence of model misspecification.

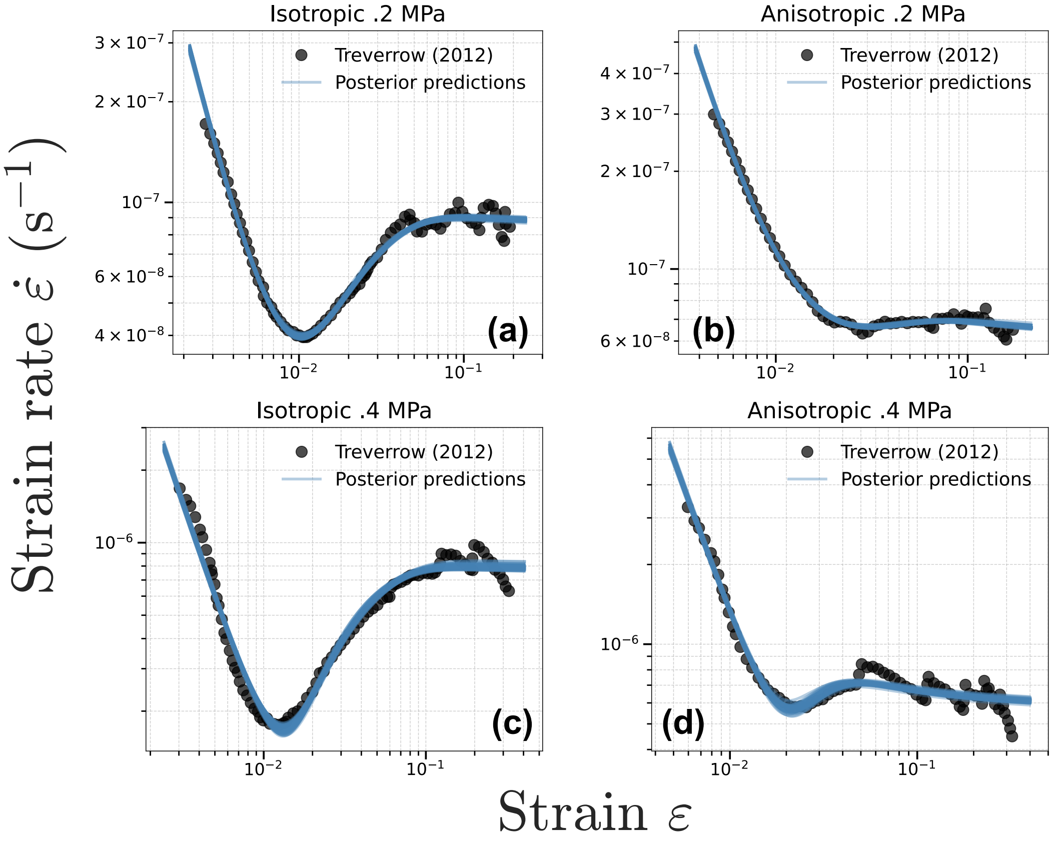


FIG. S6. Posterior predictive validation for the Treverrow *et al.* [1] 0.2,MPa dataset. Markers denote experimental strain-rate measurements, and the solid curve shows the maximum a posteriori (MAP) prediction from Eqs. (S1)–(S2). The shaded ensemble represents posterior predictive trajectories, illustrating the uncertainty in the transient evolution, including the Andrade decay, the strain-rate minimum, and the transition toward viscous flow.

Figures S6 and S7 show representative posterior predictive fits for two datasets. Each panel overlays the MAP trajectory and posterior-predictive ensemble with the experimental strain-rate measurements, together with MCMC walker traces to illustrate parameter uncertainty in the predicted curves.

## REFERENCES


[1] A. Treverrow, W. F. Budd, T. H. Jacka, and R. C. Warner, J. Glaciol. **58**, 301–314 (2012).

[2] T. H. Jacka, Cold Reg. Sci. Technol. **10**, 31 (1984).

[3] T. H. Jacka and M. Maccagnan, Cold Reg. Sci. Technol. **8**, 269 (1984).

[4] X. Q. Gao and T. H. Jacka, J. Phys. Colloq. **48**, C1 (1987).

[5] R. M. Christensen, *Theory of viscoelasticity*, 2nd ed. (Courier Corporation, 1982).

[6] C. Van der Veen and I. Whillans, Cold Reg. Sci. Technol. **22**, 171 (1994).

[7] G. P. Rigsby, J. Glaciol. **3**, 589 (1960).

[8] N. Azuma and A. Higashi, Ann. Glaciol. **6**, 130 (1985).

[9] F. Gillet-Chaulet, O. Gagliardini, J. Meyssonnier, M. Montagnat, and O. Castelnau, J. Glaciol. **51**, 3 (2005).

[10] F. Gillet-Chaulet, O. Gagliardini, J. Meyssonnier, T. Zwinger, and J. Ruokolainen, J. Non-Newton. Fluid Mech. **134**, 33 (2006).

[11] J. Weertman, Annu. Rev. Earth Planet. Sci. **11**, 215 (1983).

[12] D. Foreman-Mackey, D. W. Hogg, D. Lang, and J. Goodman, Publ. Astron. Soc. Pac. **125**, 306 (2013).

[13] R. Ran, S. Pradeep, S. Kosgodagan Acharige, B. C. Blackwell, C. Kammer, D. J. Jerolmack, and P. E. Arratia, J. Rheol. **67**, 241 (2023).

[14] R. Ran, J. C. Burton, S. Kumar, S. Bhamla, A. R. Dillman, and V. M. Ortega-Jimenez, Proc. Natl. Acad. Sci. U.S.A. **122**, e2503555122 (2025).

# APPENDIX A: TABLES AND ADDITIONAL FIGURES

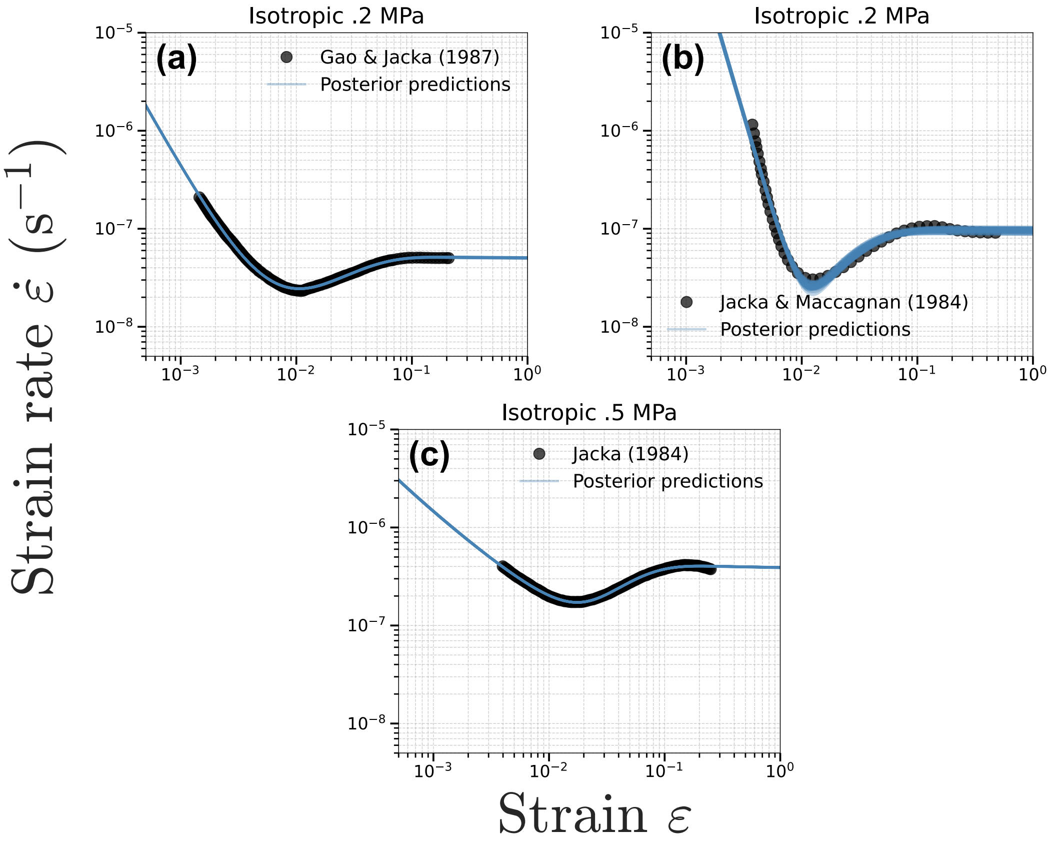


FIG. S7. Posterior predictive validation for the Gao and Jacka [4] 0.2,MPa, Jacka and Maccagnan [3] 0.2,MPa, and Jacka [2] 0.5,MPa datasets. Experimental strain-rate data (markers) are shown together with the MAP trajectories (solid curves) and posterior predictive ensembles quantifying the uncertainty in the transient creep response. Across all three datasets, the inferred parameters reproduce the primary Andrade decay, the emergence and location of the strain-rate minimum, and the late-time viscous asymptote.

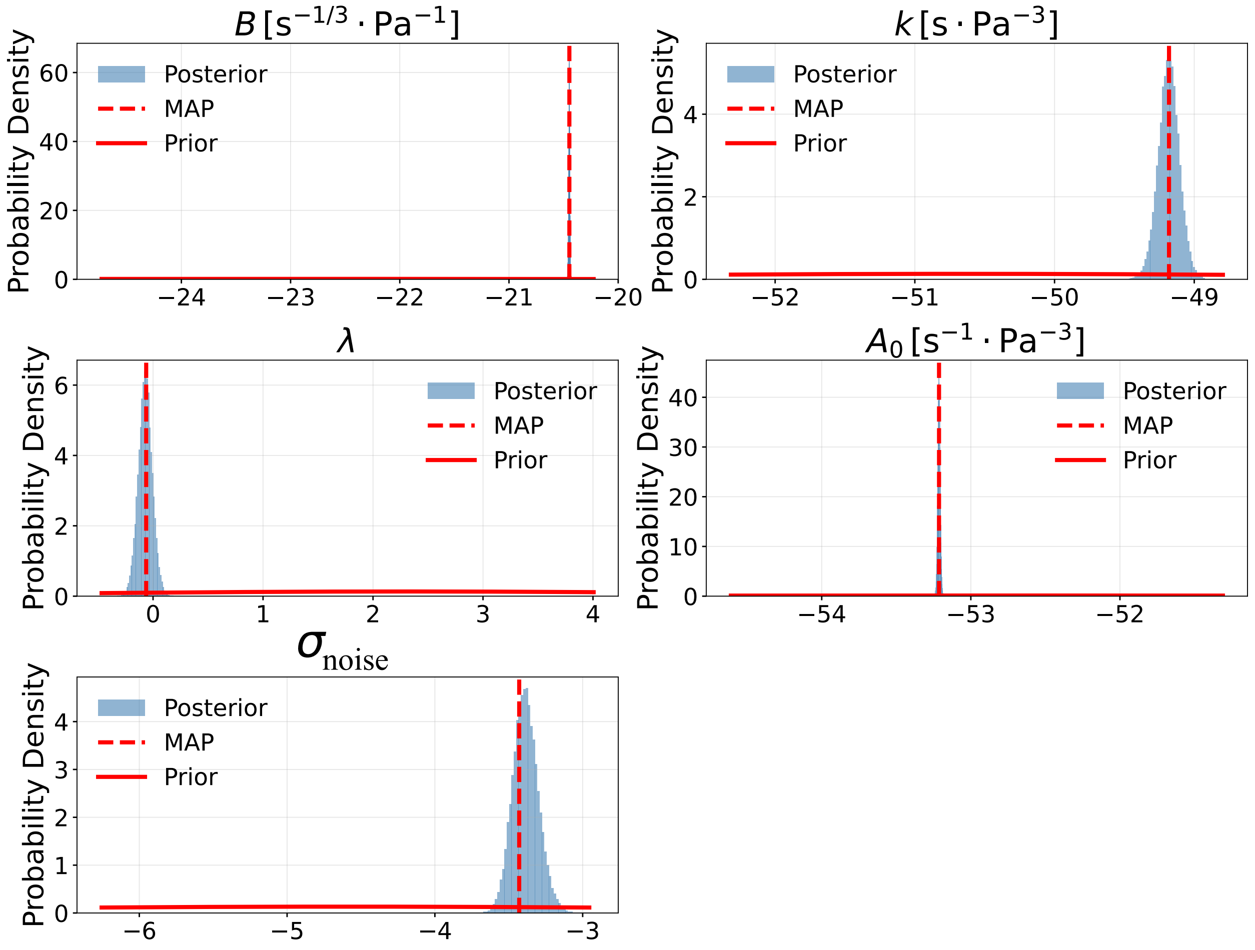


FIG. S8. Prior and posterior distributions of the free parameters inferred from the MCMC fit for the anisotropic .2 MPa experiment from Treverrow *et al.* [1]. Red dashed lines indicate MAP values. Parameters are shown in log-space where appropriate, with physical units given in brackets.

TABLE S1. Common lognormal priors used for MCMC fits for Treverrow *et al.* [1]. Each parameter is defined in log-space with standard deviation $\sigma = 3.0$. The stress exponent used for the fits are $p = 3$

| Parameter | Prior |
|---|---|
| $\log_{10} B$ | Lognormal($\mu = \log 1.0{\times}10^{-9}$, $\sigma = 3.0$) |
| $\log_{10} k$ | Lognormal($\mu = \log 1.0{\times}10^{-21}$, $\sigma = 3.0$) |
| $\log_{10} A_0$ | Lognormal($\mu = \log 1.0{\times}10^{-23}$, $\sigma = 3.0$) |
| $\log_{10} \lambda$ | Lognormal($\mu = \log 1.0{\times}10^{1}$, $\sigma = 3.0$) |
| $\log_{10} \sigma_{\mathrm{noise}}$ | Lognormal($\mu = \log 1.0{\times}10^{-1}$, $\sigma = 3.0$) |

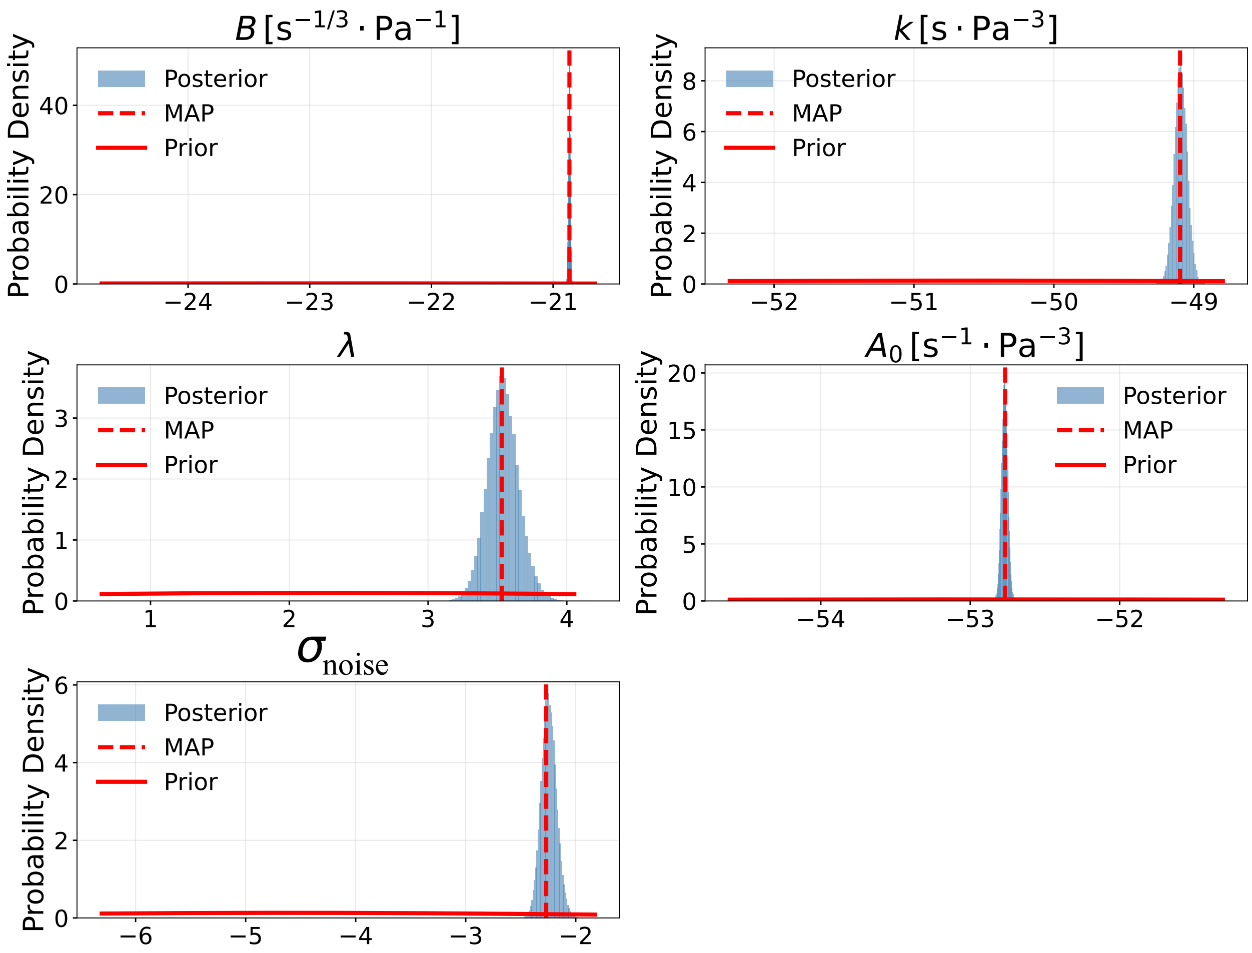


FIG. S9. Prior and posterior distributions of the free parameters inferred from the MCMC fit for the isotropic .4 MPa experiment from Treverrow *et al.* [1]. Red dashed lines indicate MAP values. Parameters are shown in log-space where appropriate, with physical units given in brackets.

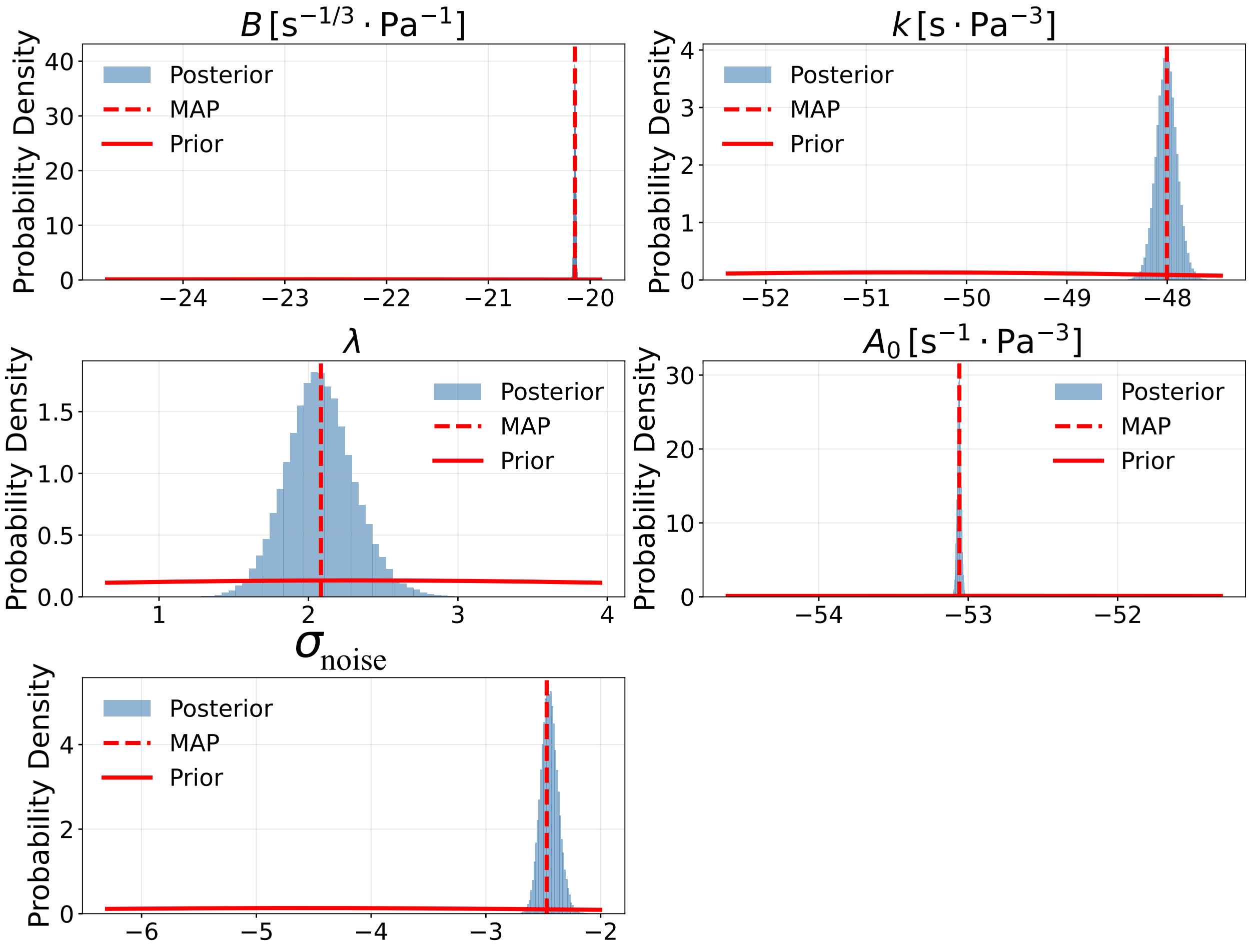


FIG. S10. Prior and posterior distributions of the free parameters inferred from the MCMC fit for the anisotropic .4 MPa experiment from Treverrow *et al.* [1]. Red dashed lines indicate MAP values. Parameters are shown in log-space where appropriate, with physical units given in brackets.

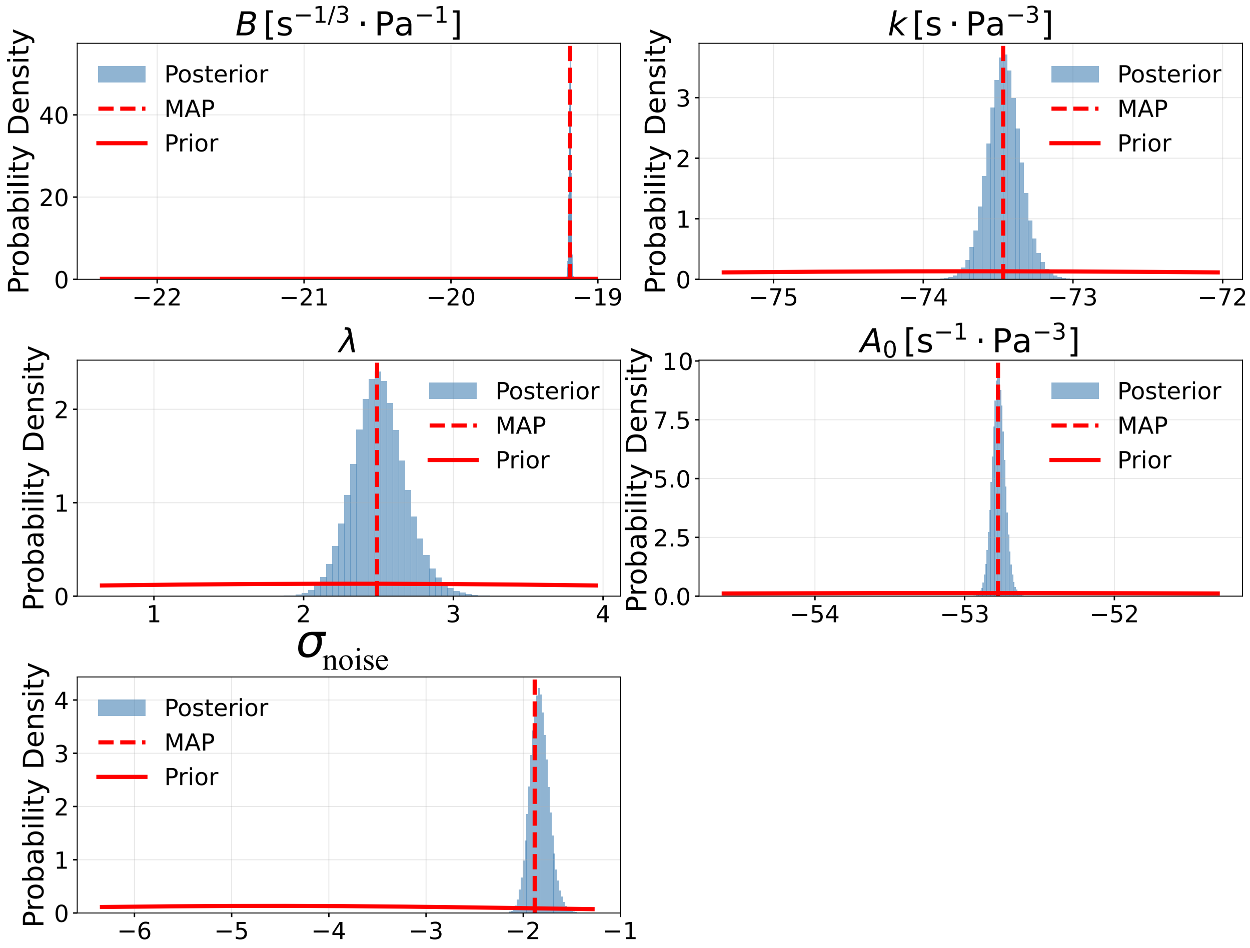


FIG. S11. Prior and posterior distributions of the free parameters inferred from the MCMC fit for the isotropic .2 MPa experiment from Jacka and Maccagnan [3]. Red dashed lines indicate MAP values. Parameters are shown in log-space where appropriate, with physical units given in brackets.

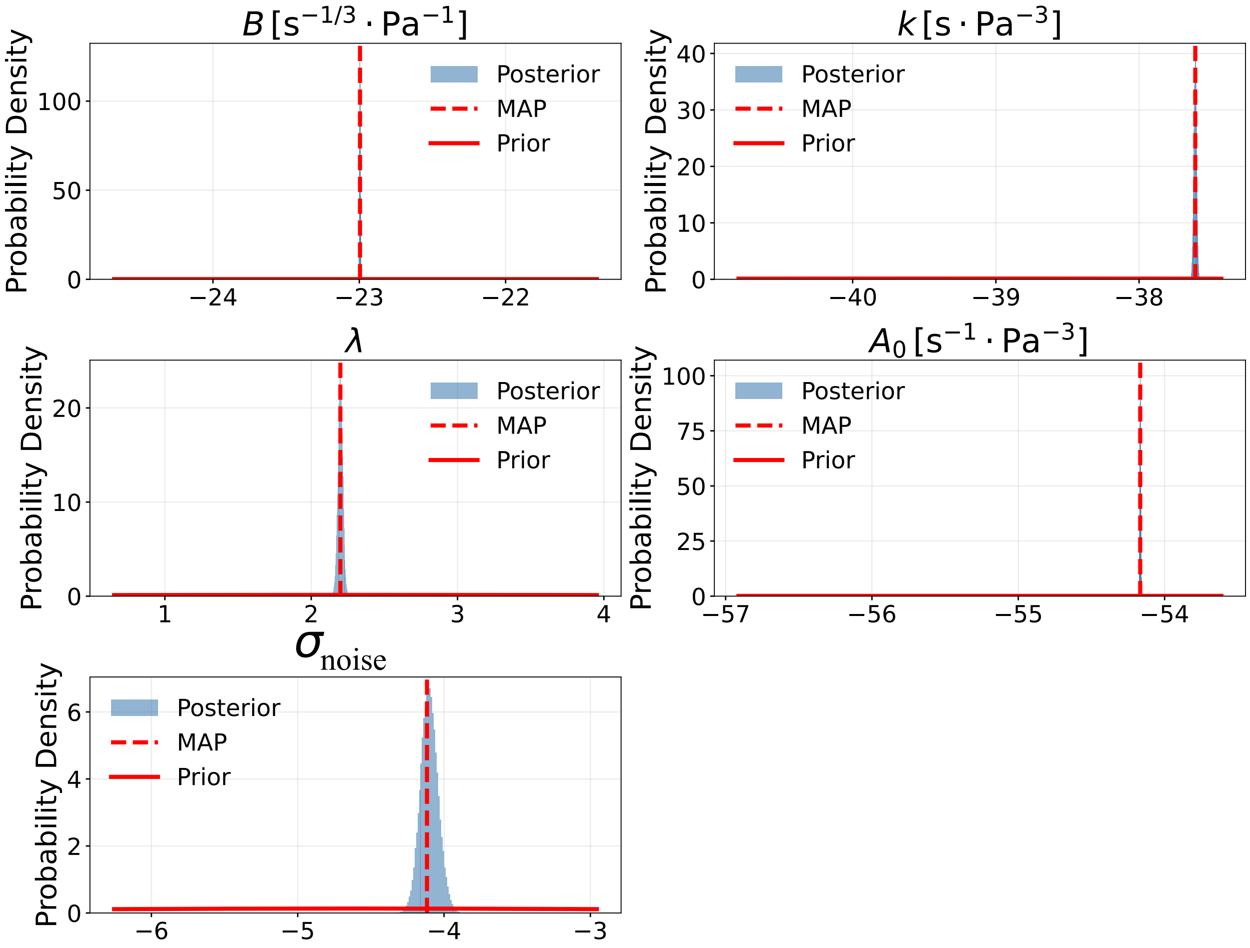


FIG. S12. Prior and posterior distributions of the free parameters inferred from the MCMC fit for the isotropic .5 MPa experiment from Jacka [2]. Red dashed lines indicate MAP values. Parameters are shown in log-space where appropriate, with physical units given in brackets.

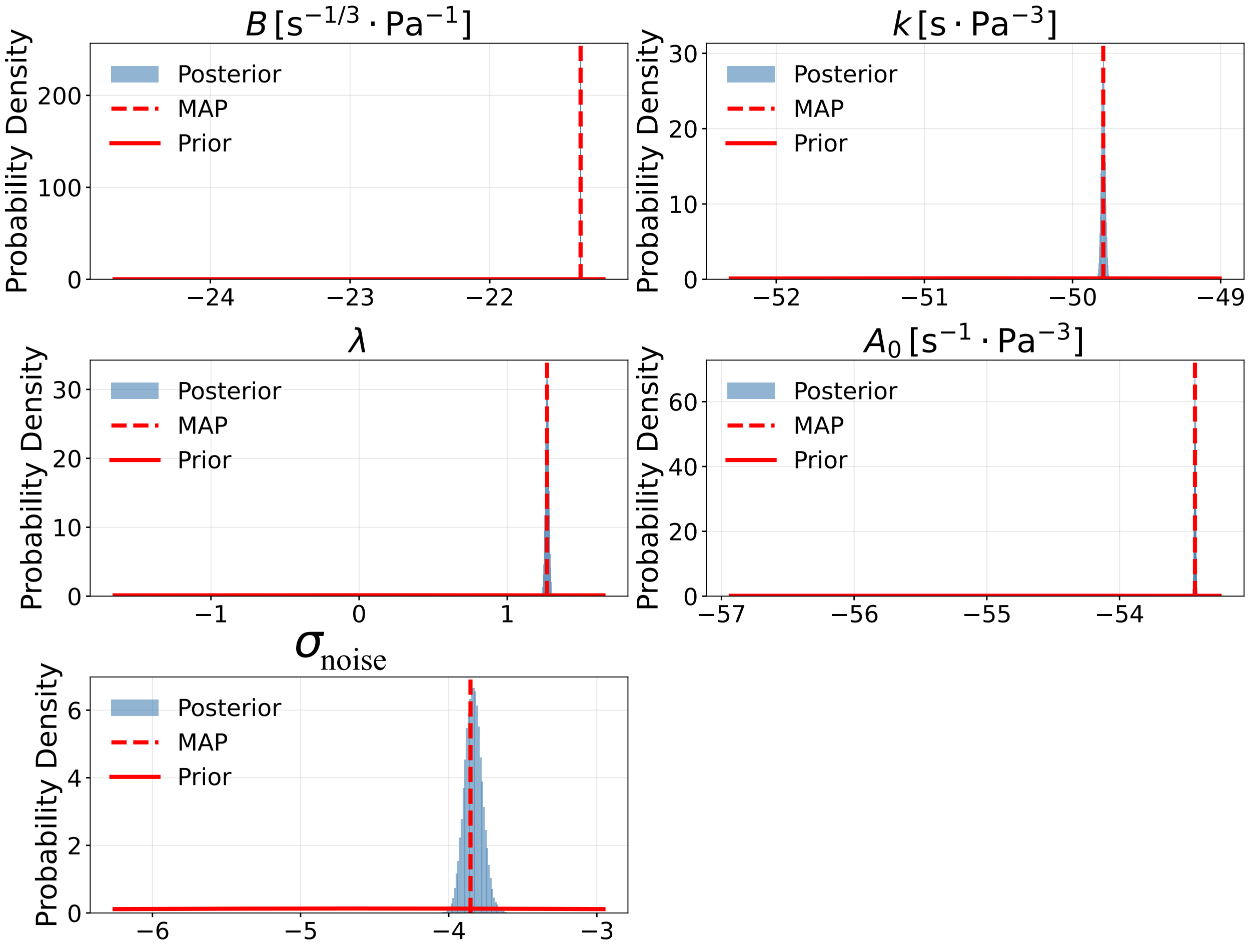


FIG. S13. Prior and posterior distributions of the free parameters inferred from the MCMC fit for the isotropic .2 MPa experiment from Gao and Jacka [4]. Red dashed lines indicate MAP values. Parameters are shown in log-space where appropriate, with physical units given in brackets.

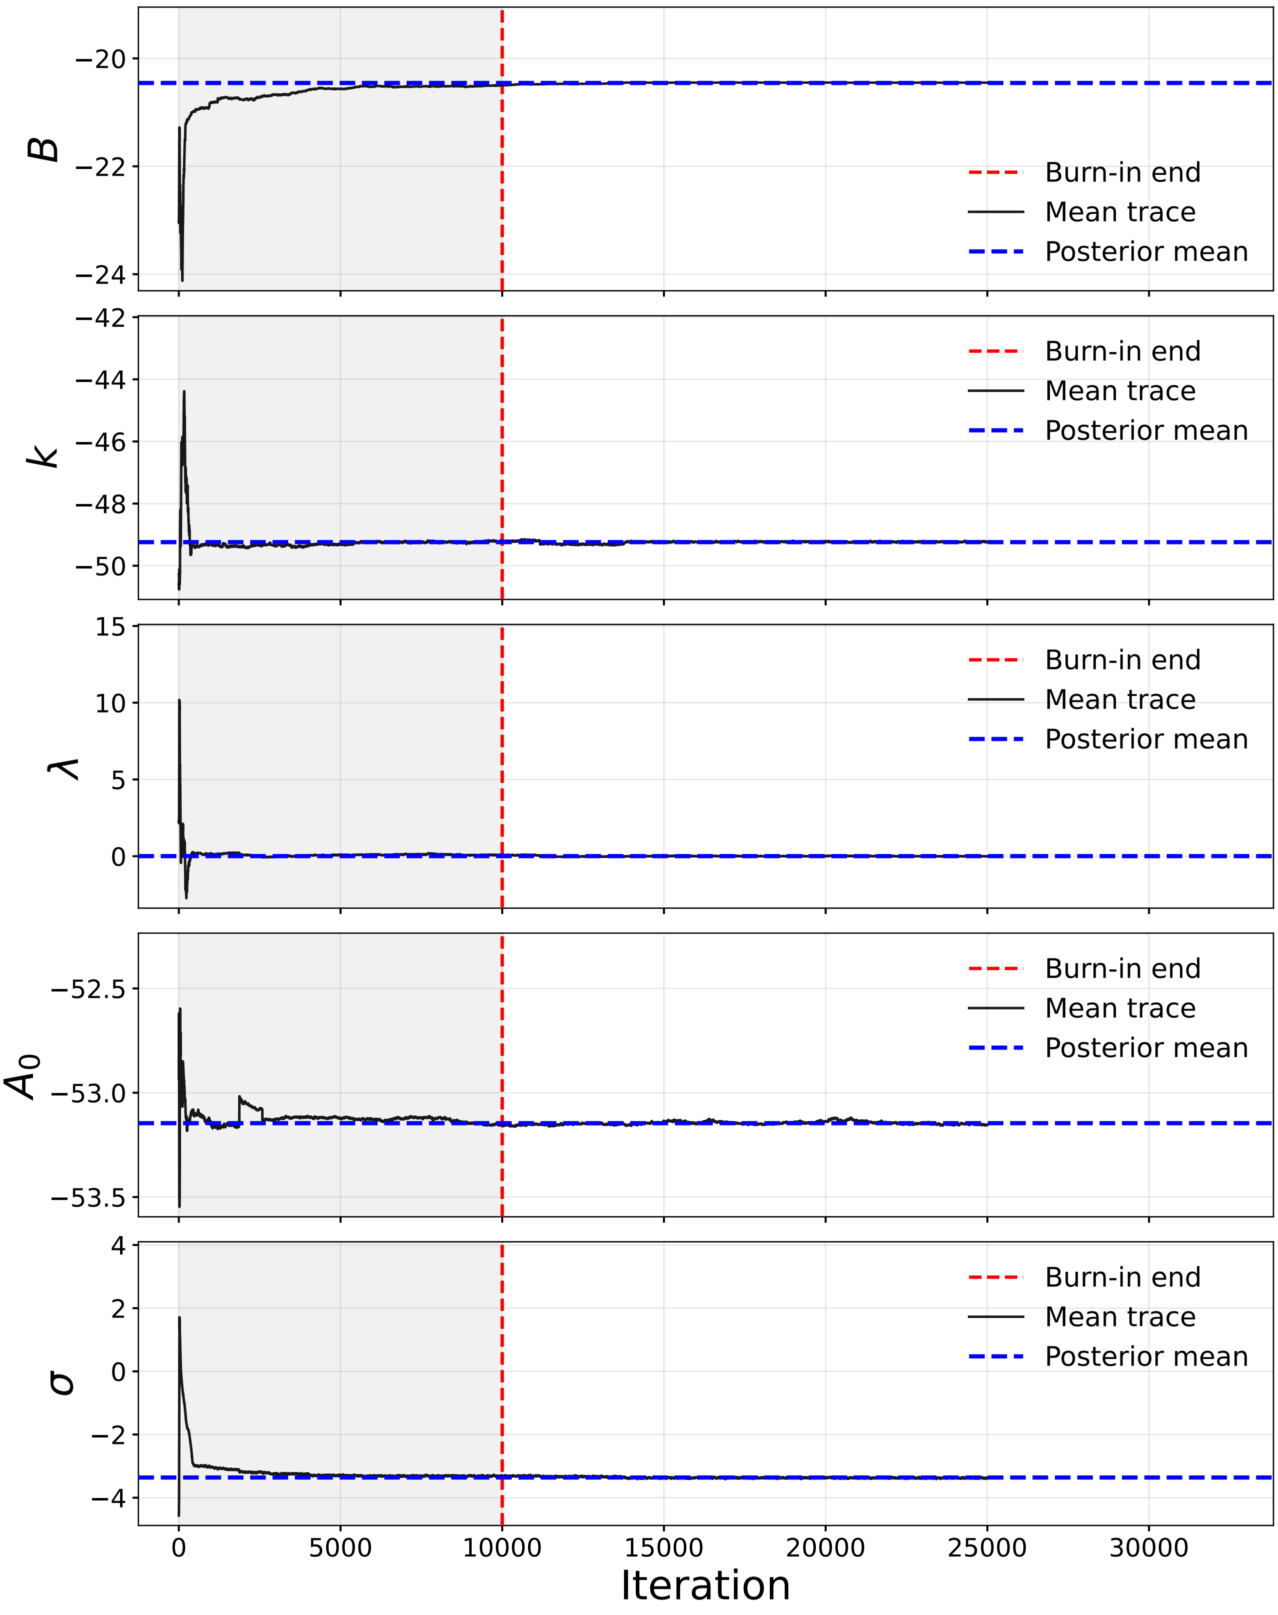


FIG. S14. Free parameters traces from the MCMC fit for the anisotropic .2 MPa experiment from Treverrow *et al.* [1]. Red dashed lines indicate MAP values. Parameters are shown in log-space where appropriate, with physical units given in brackets.

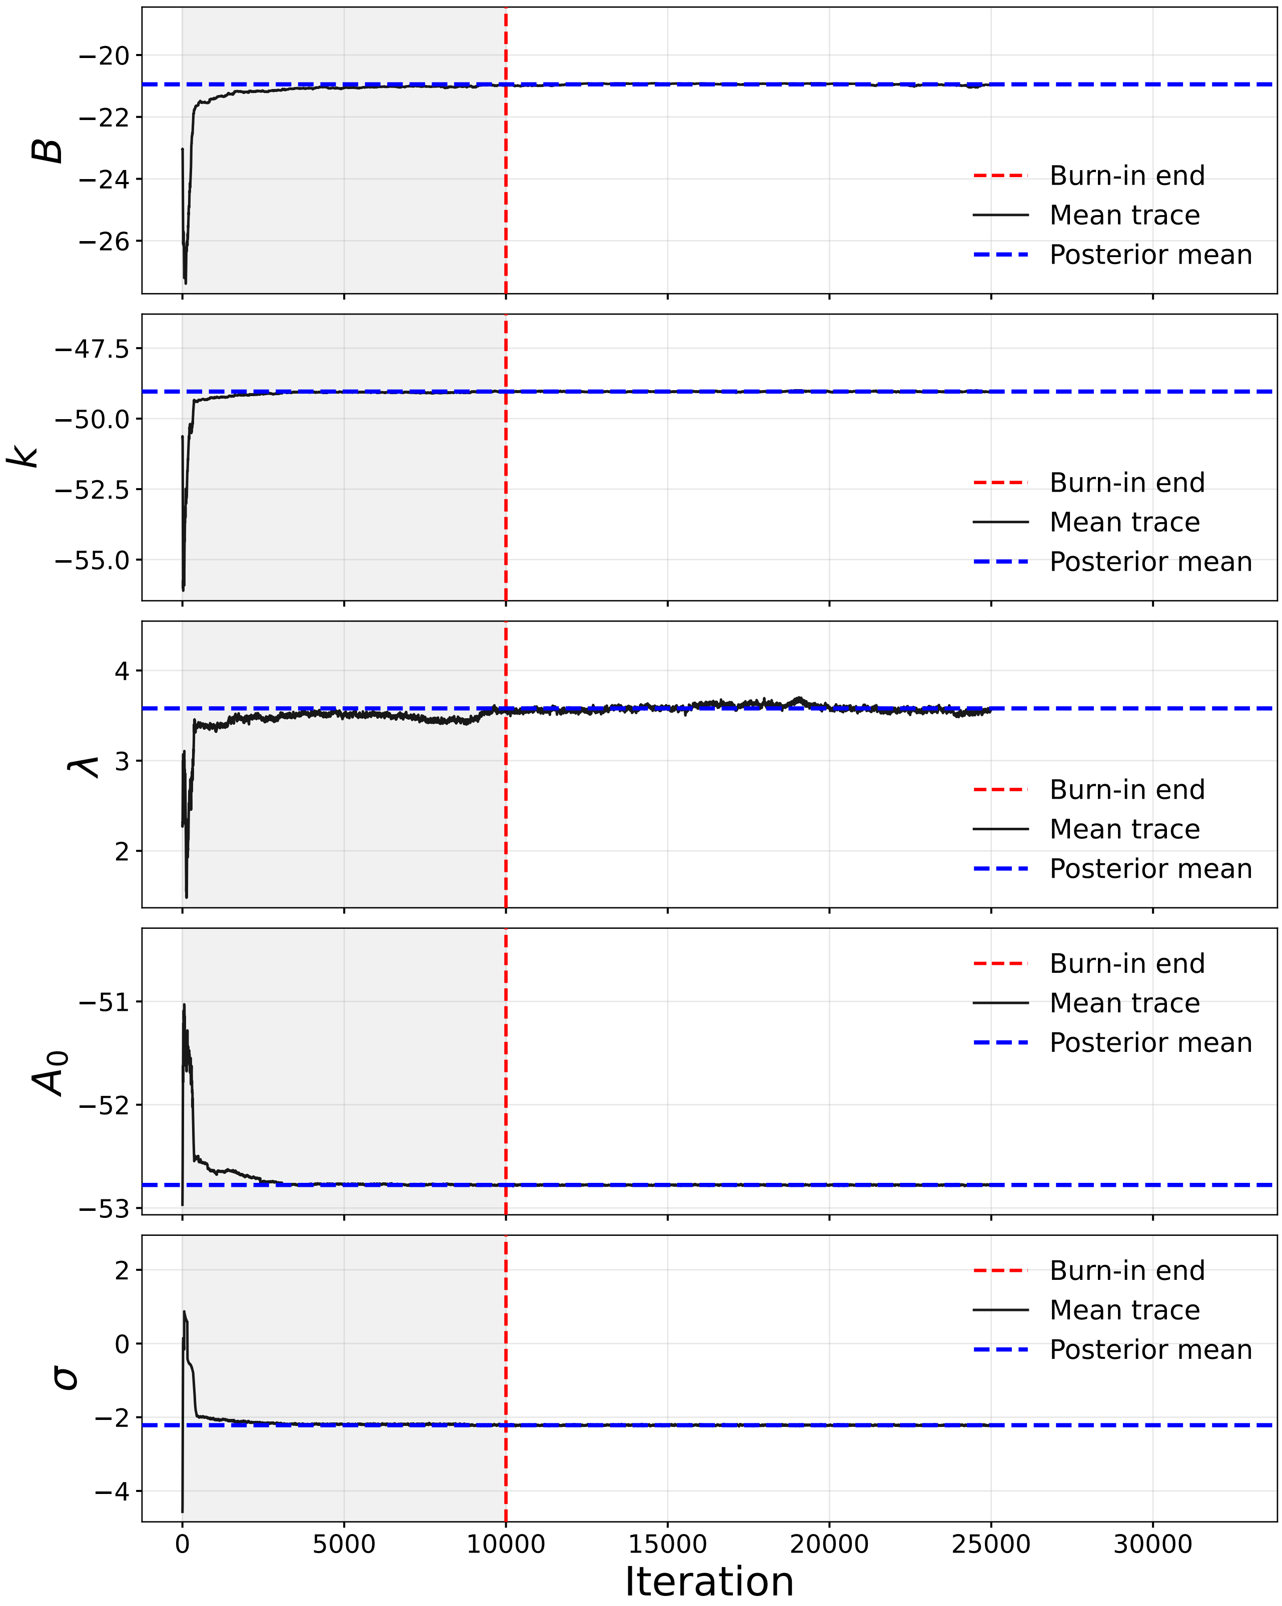


FIG. S15. Free parameters traces from the MCMC fit for the isotropic .4 MPa experiment from Treverrow *et al.* [1]. Red dashed lines indicate MAP values. Parameters are shown in log-space where appropriate, with physical units given in brackets.

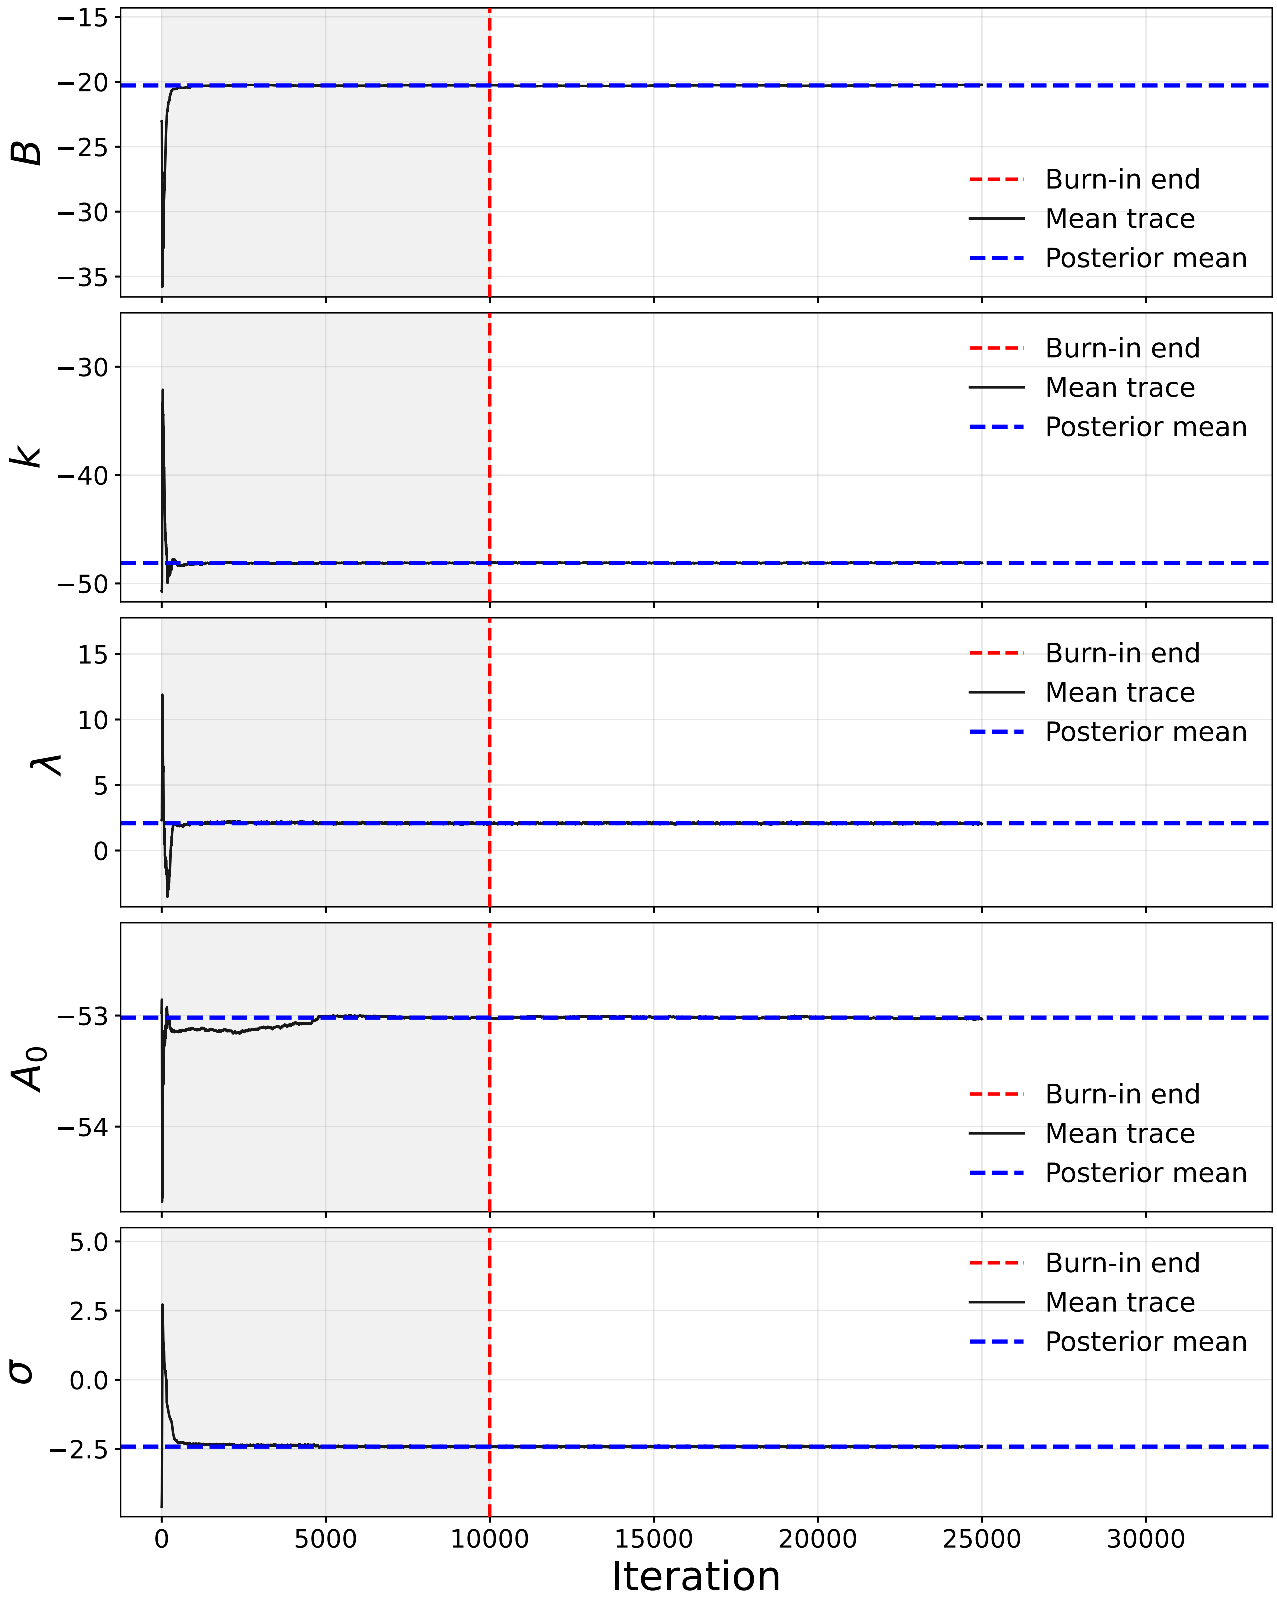


FIG. S16. Free parameters traces from the MCMC fit for the anisotropic .4 MPa experiment from Treverrow *et al.* [1]. Red dashed lines indicate MAP values. Parameters are shown in log-space where appropriate, with physical units given in brackets.

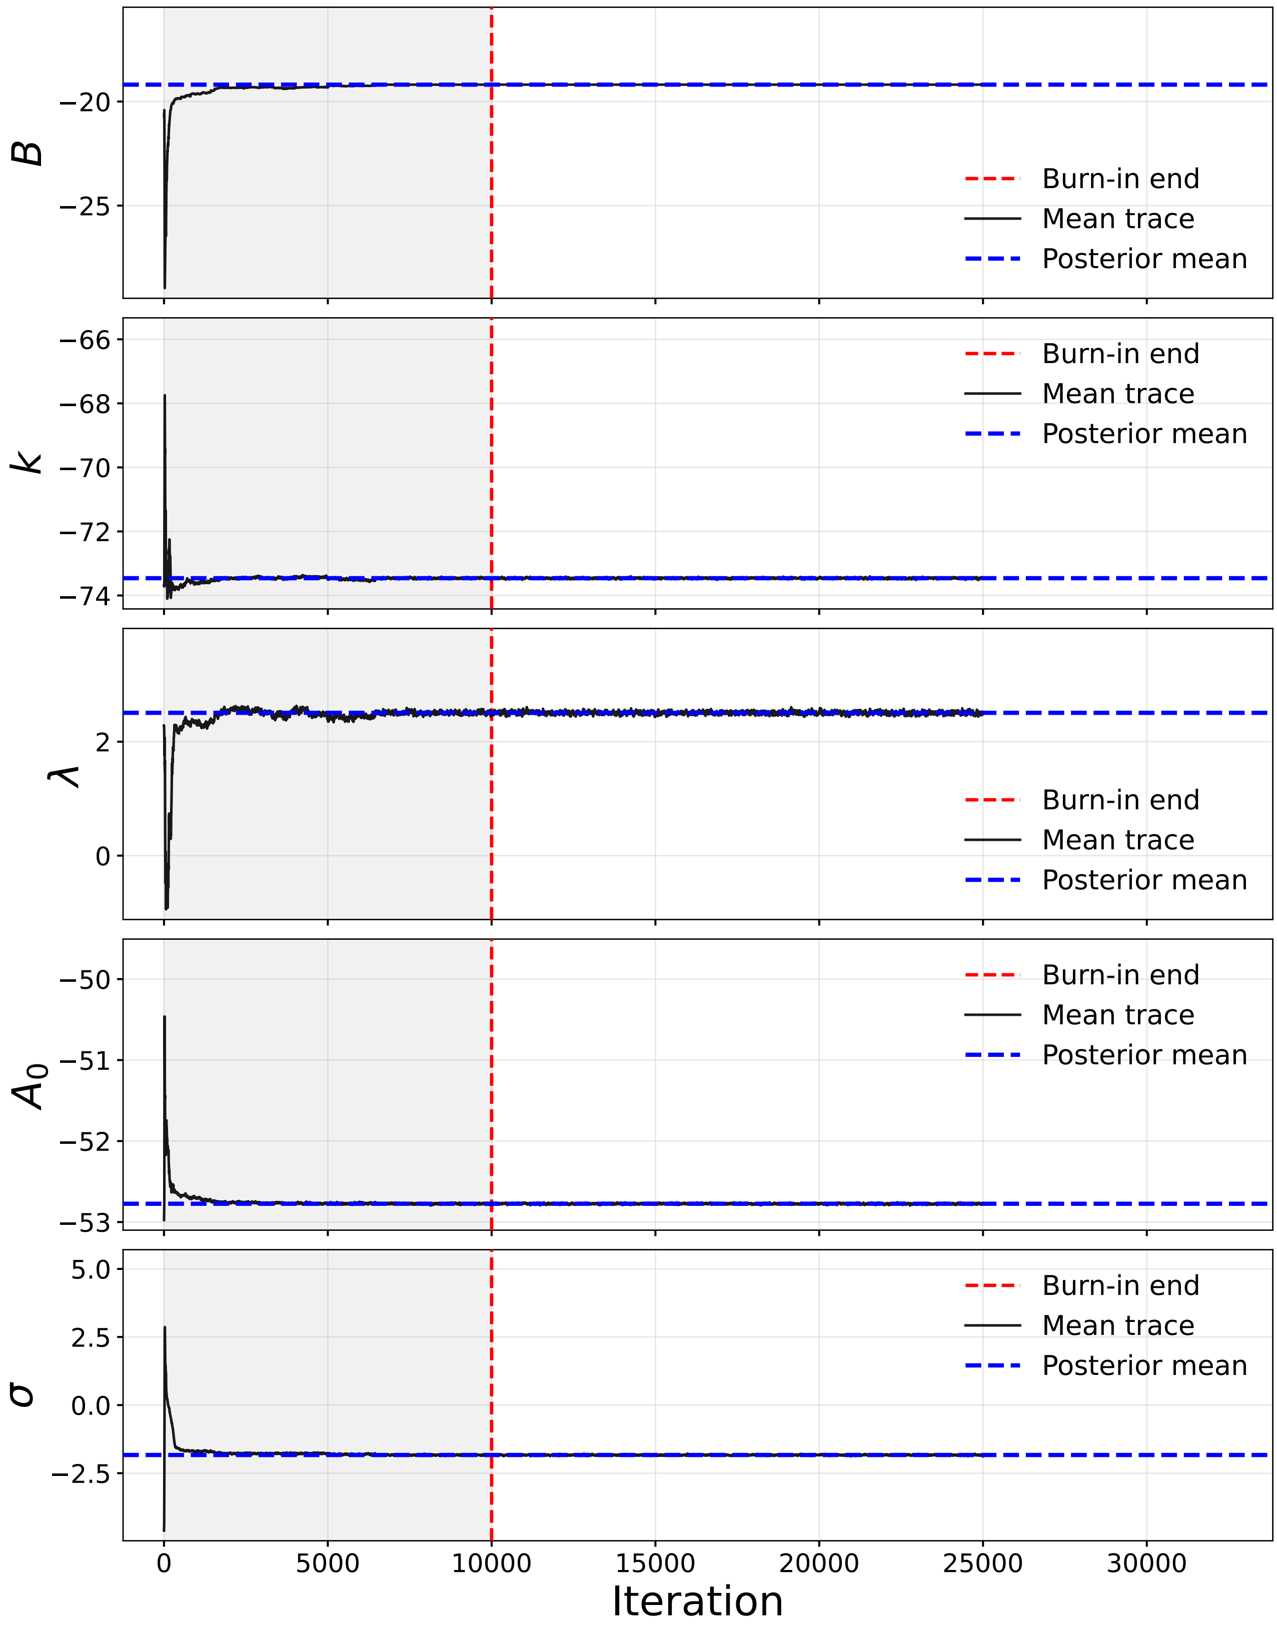


FIG. S17. Free parameters traces from the MCMC fit for the isotropic .2 MPa experiment from Jacka and Maccagnan [3]. Red dashed lines indicate MAP values. Parameters are shown in log-space where appropriate, with physical units given in brackets.

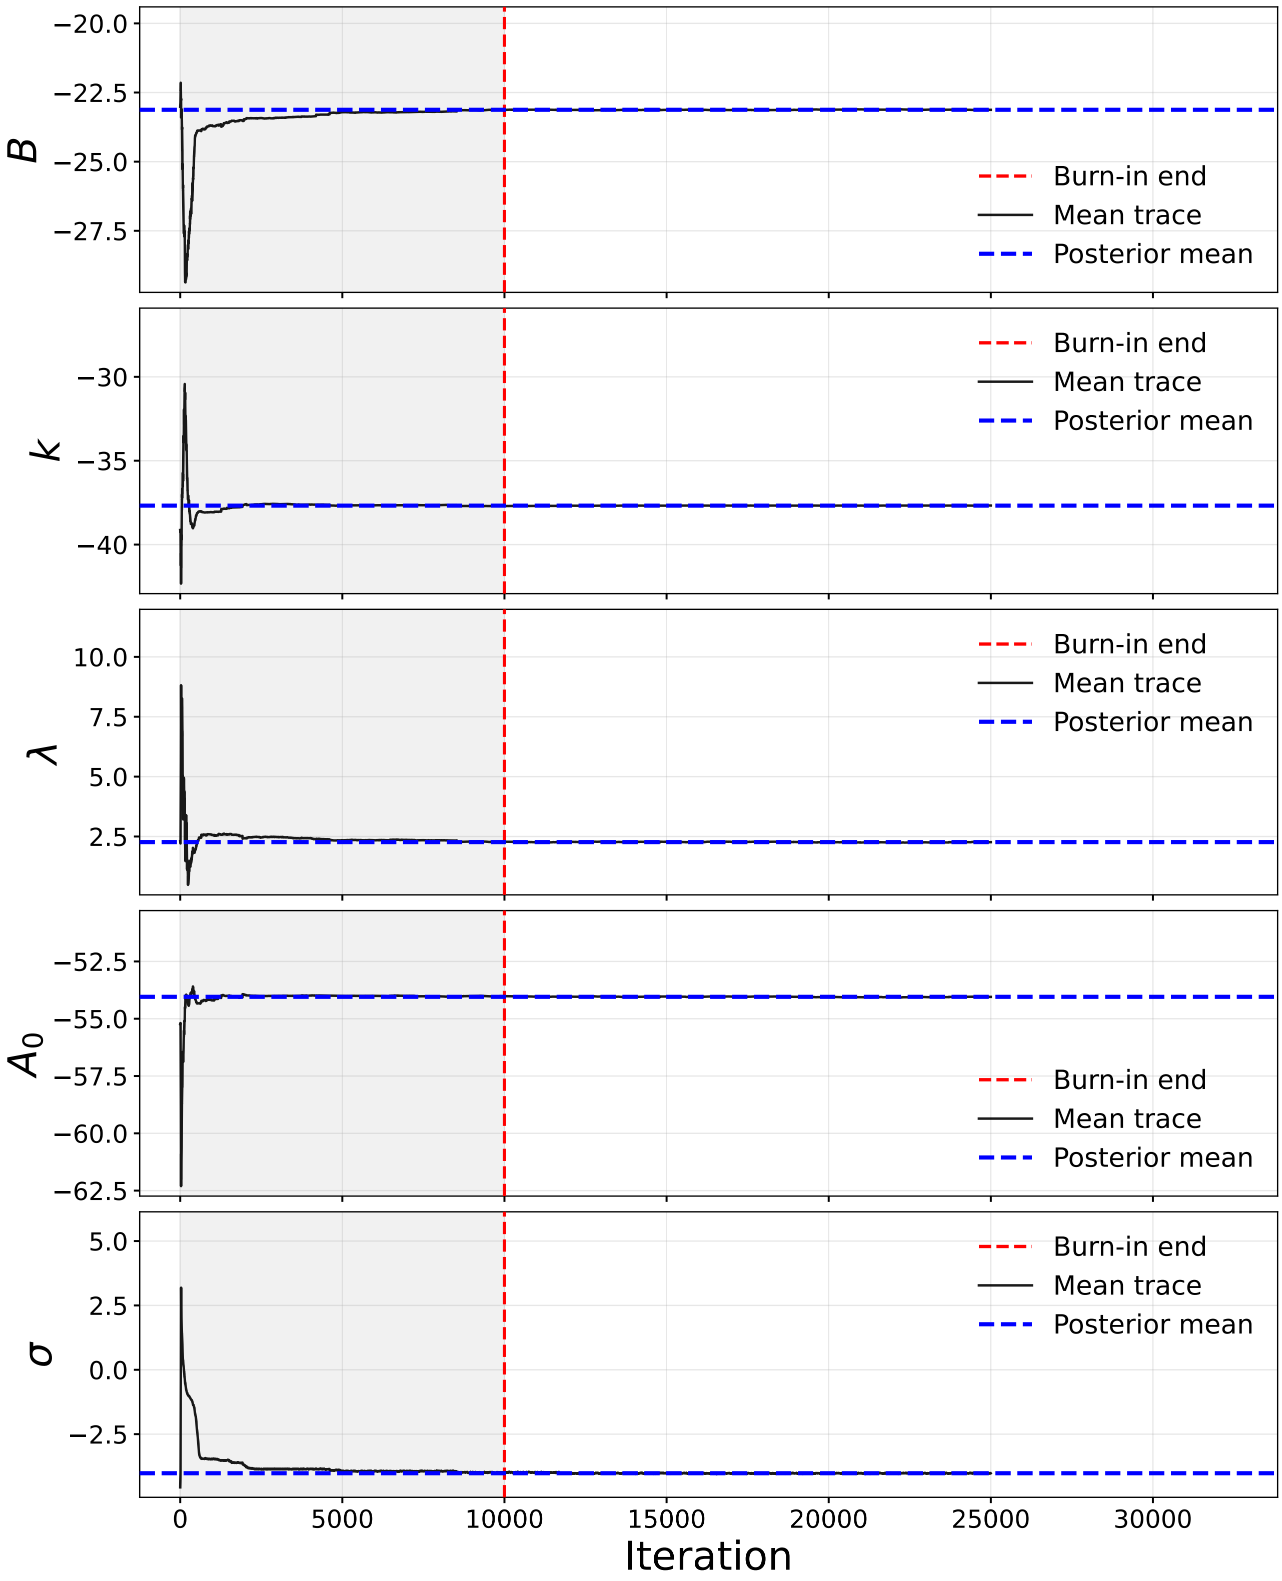


FIG. S18. Free parameters traces from the MCMC fit for the isotropic .5 MPa experiment from Jacka [2]. Red dashed lines indicate MAP values. Parameters are shown in log-space where appropriate, with physical units given in brackets.

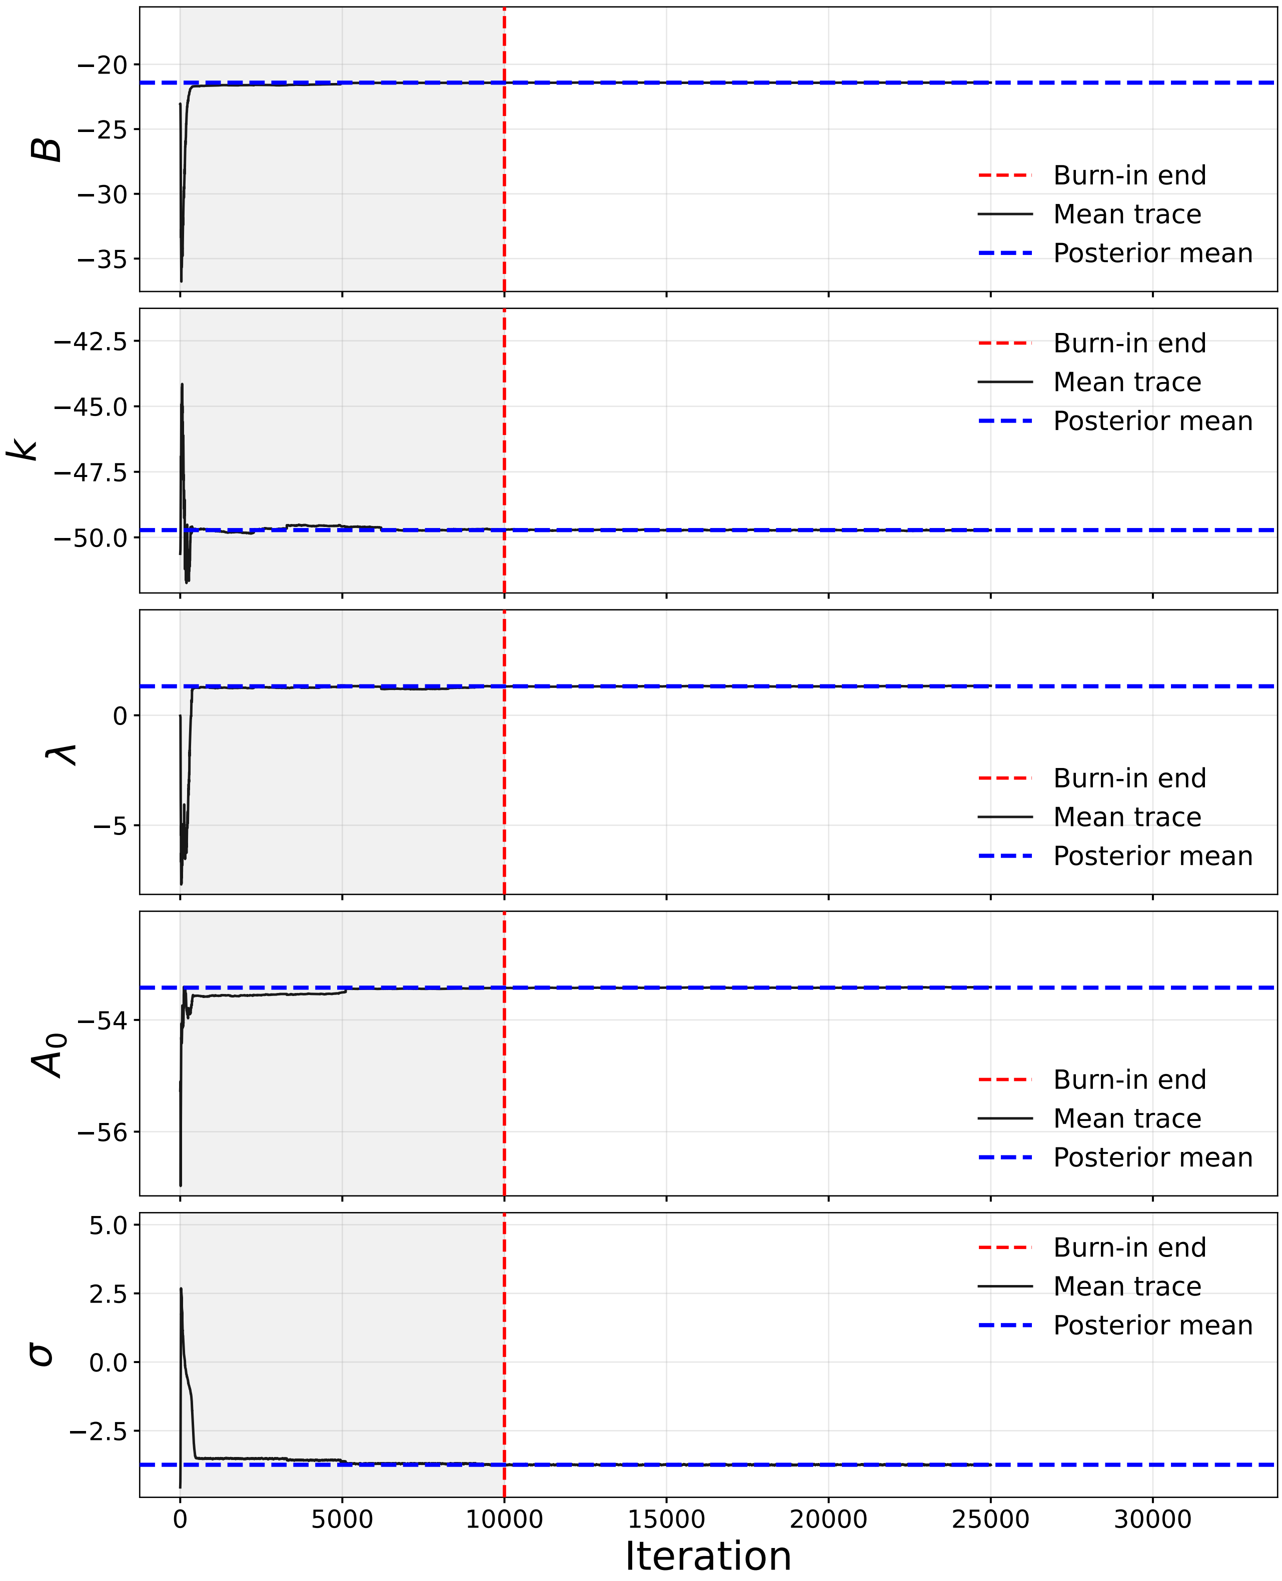


FIG. S19. Free parameters traces from the MCMC fit for the isotropic .2 MPa experiment from Gao and Jacka [4]. Red dashed lines indicate MAP values. Parameters are shown in log-space where appropriate, with physical units given in brackets.

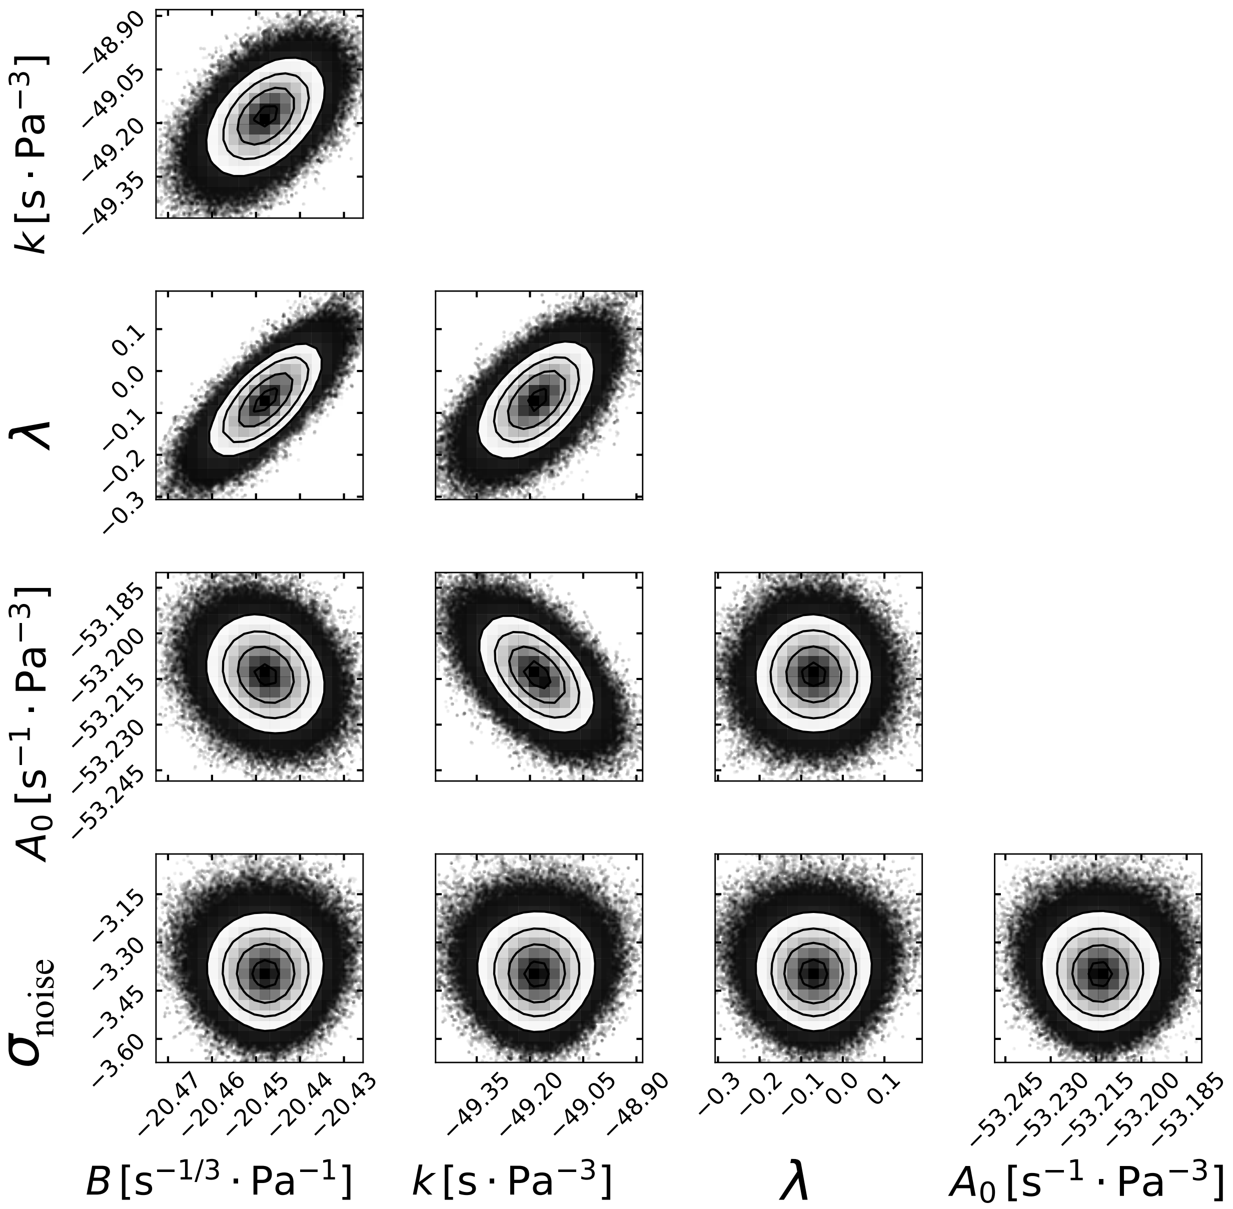


FIG. S20. Free parameters correlations from the MCMC fit for the anisotropic .2 MPa experiment from Treverrow *et al.* [1]. Red dashed lines indicate MAP values. Parameters are shown in log-space where appropriate, with physical units given in brackets.

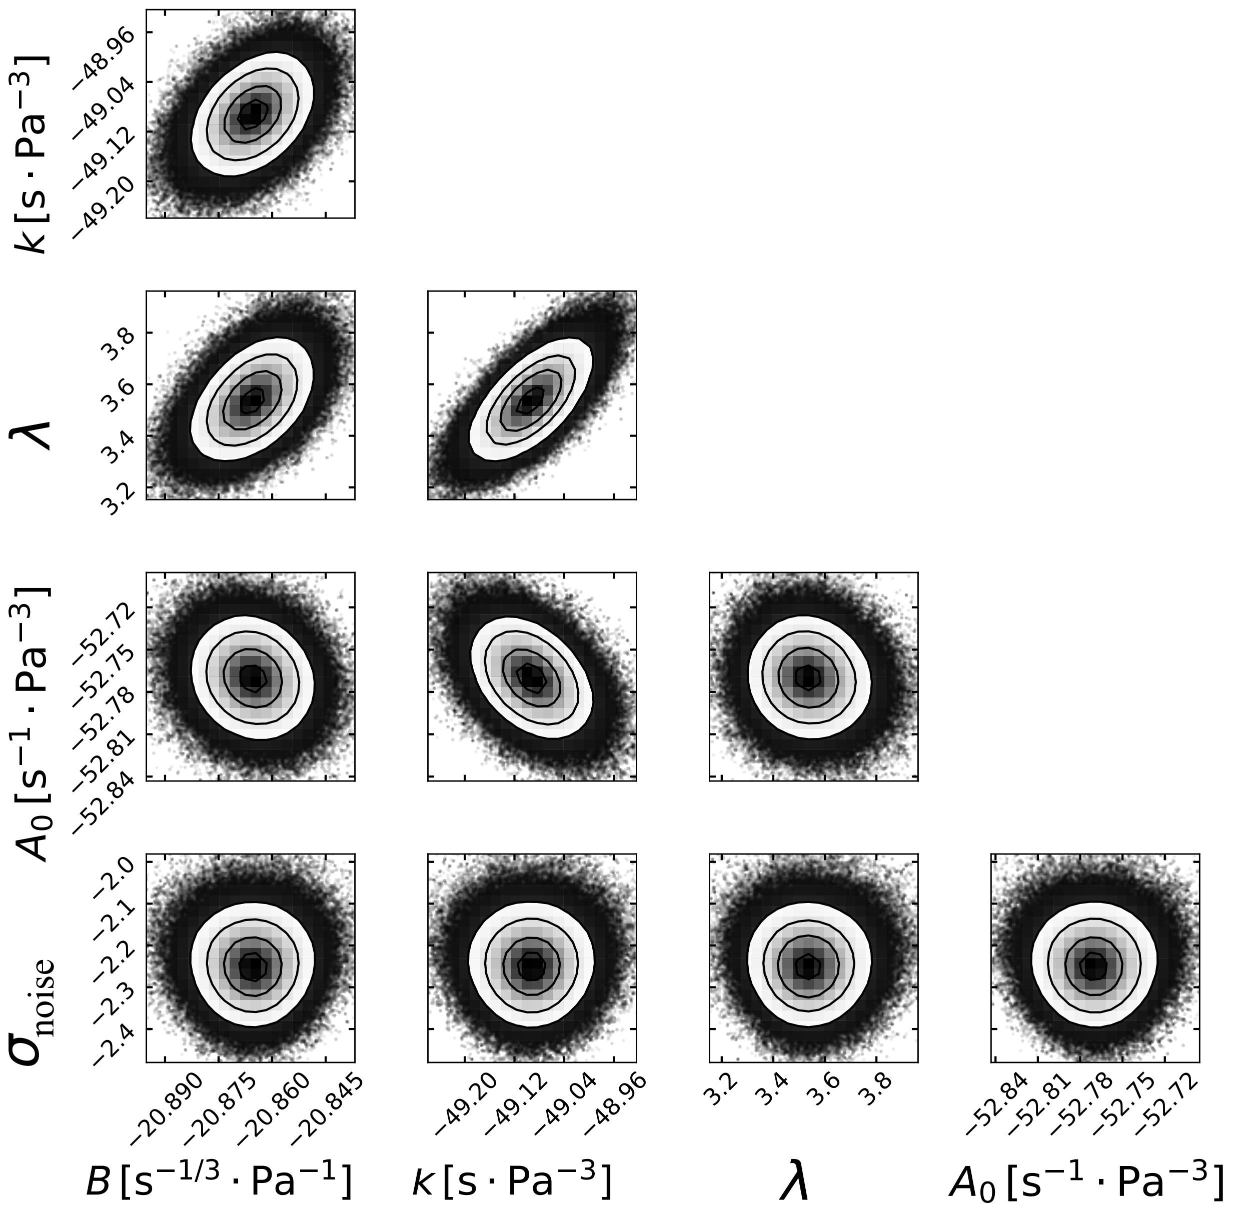


FIG. S21. Free parameters correlations from the MCMC fit for the isotropic .4 MPa experiment from Treverrow *et al.* [1]. Red dashed lines indicate MAP values. Parameters are shown in log-space where appropriate, with physical units given in brackets.

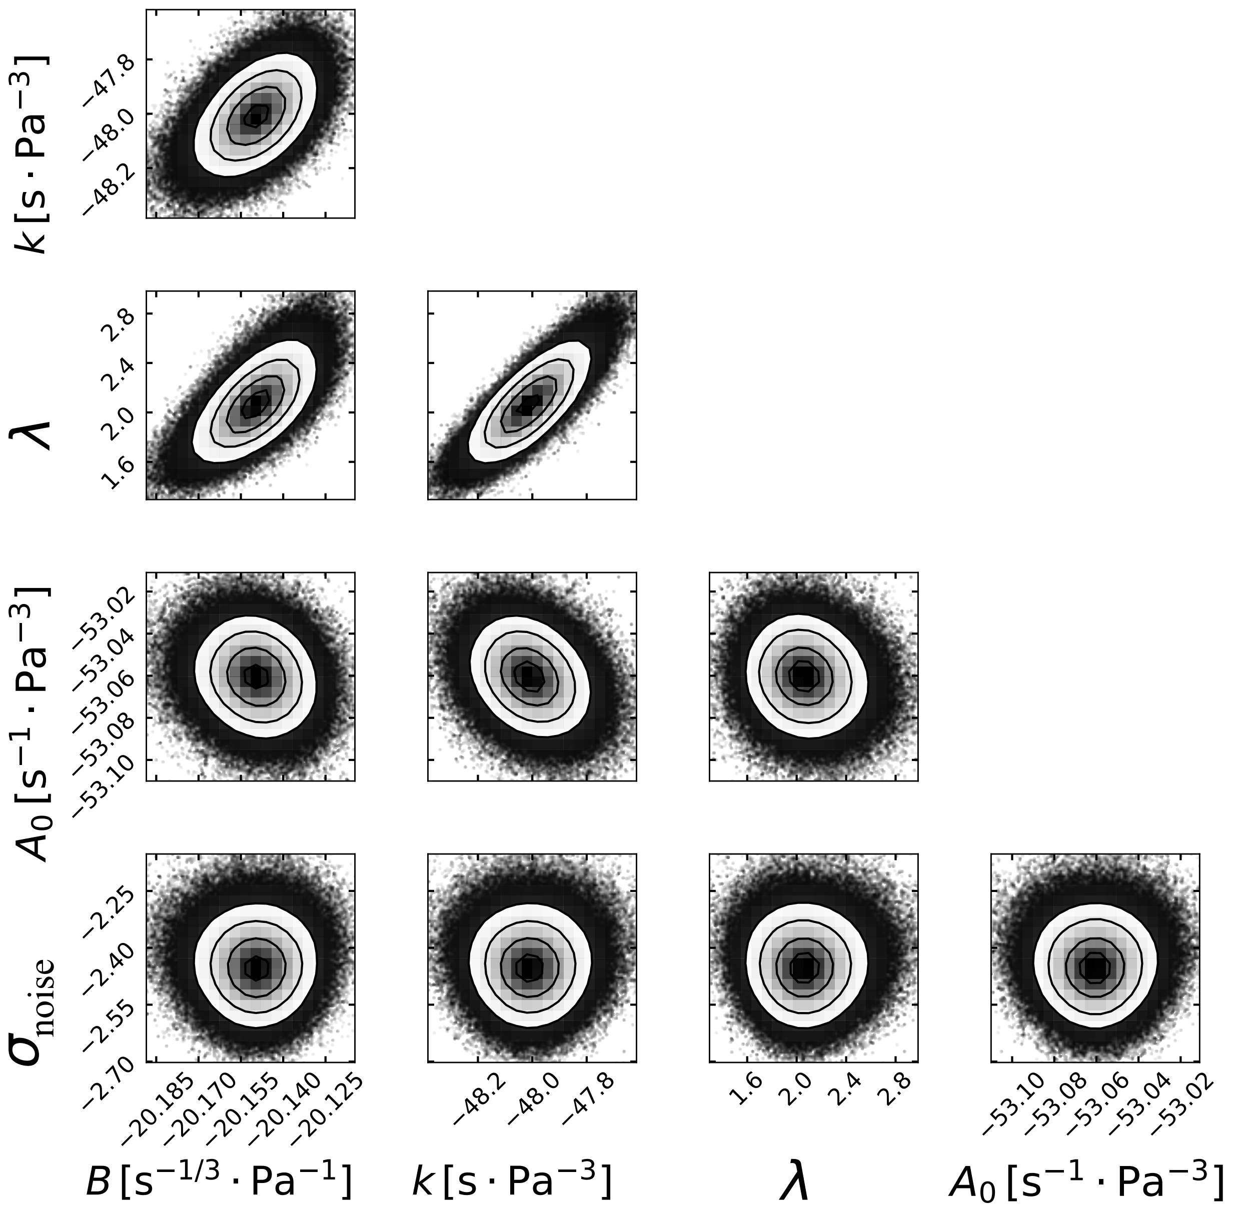


FIG. S22. Free parameters correlations from the MCMC fit for the anisotropic .4 MPa experiment from Treverrow *et al.* [1]. Red dashed lines indicate MAP values. Parameters are shown in log-space where appropriate, with physical units given in brackets.

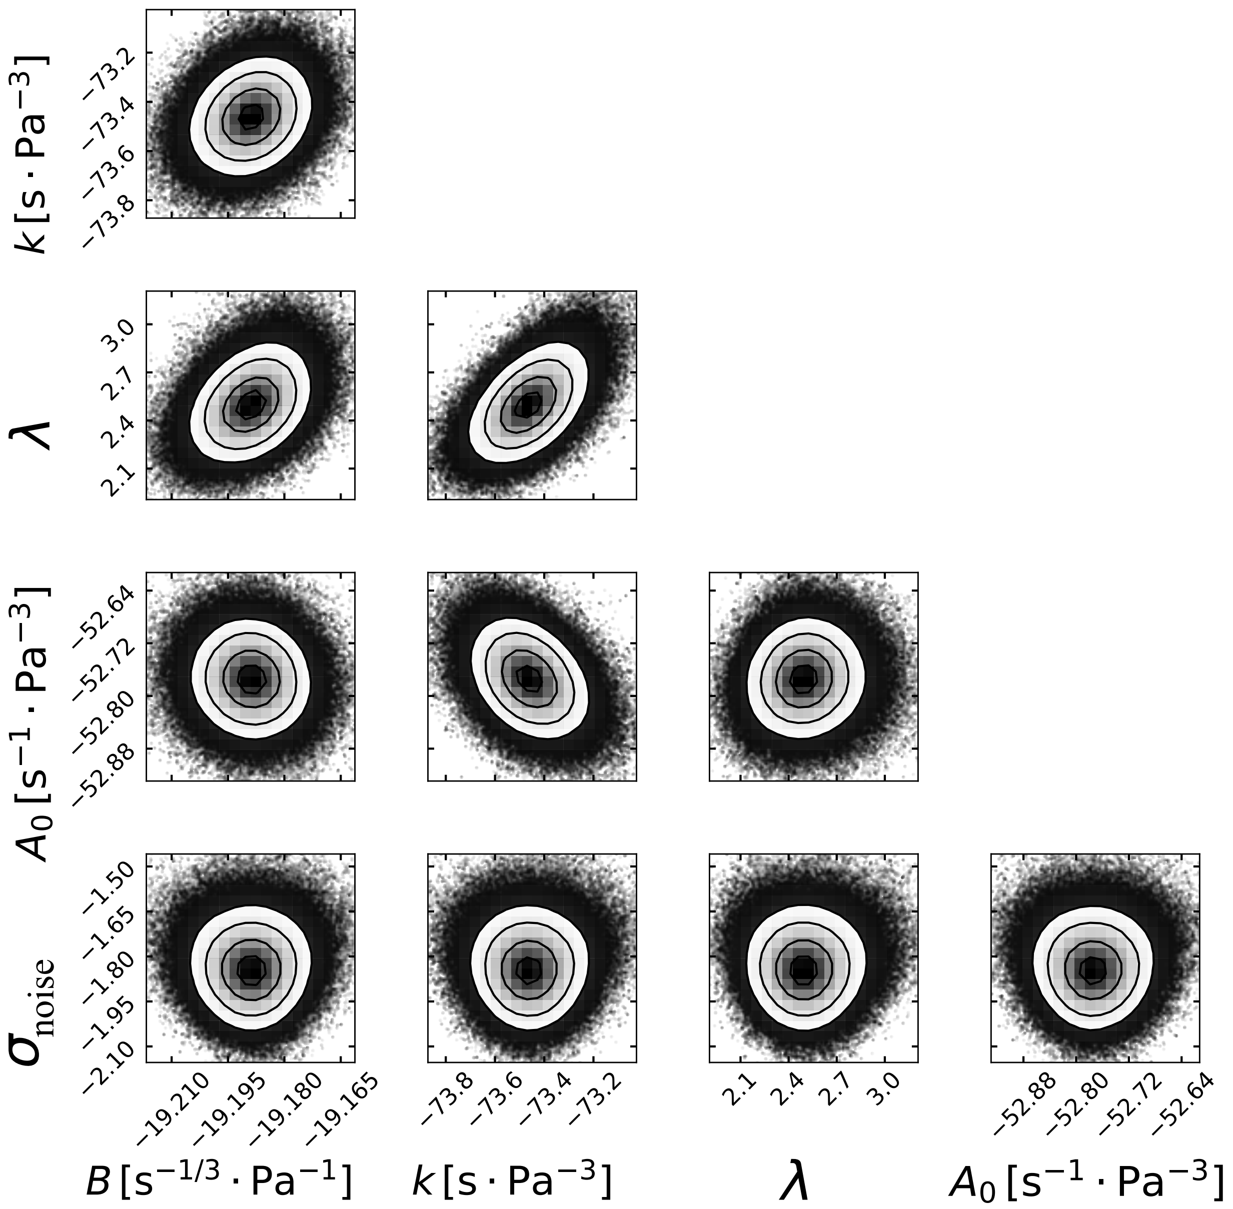


FIG. S23. Free parameters correlations from the MCMC fit for the isotropic .2 MPa experiment from Jacka and Maccagnan [3]. Red dashed lines indicate MAP values. Parameters are shown in log-space where appropriate, with physical units given in brackets.

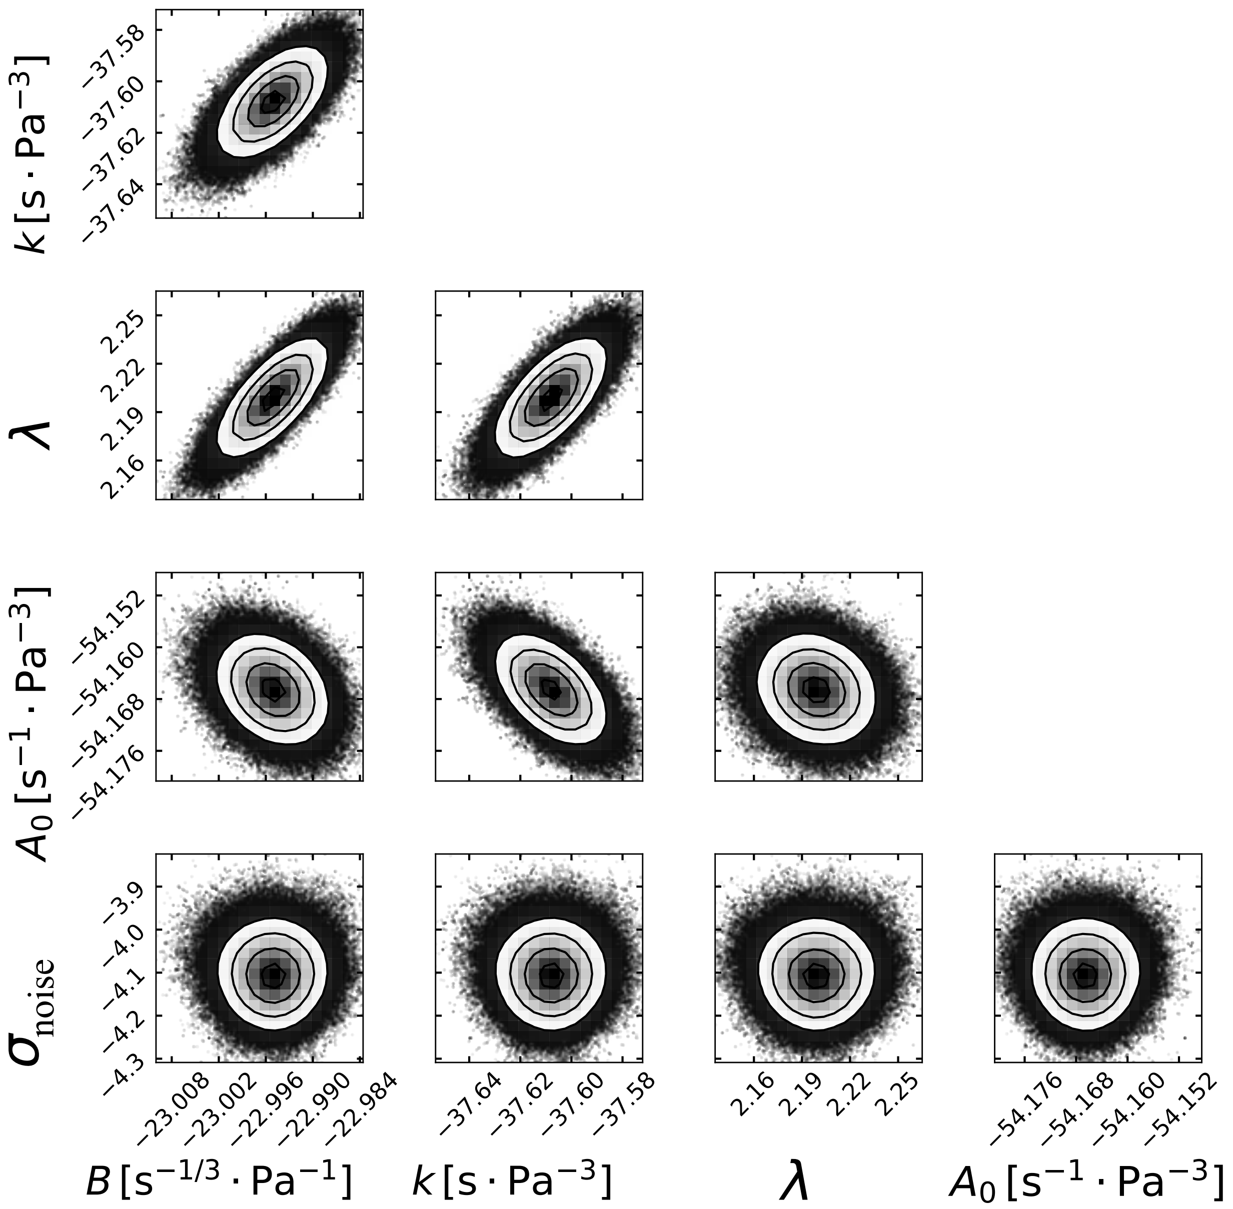


FIG. S24. Free parameters correlations from the MCMC fit for the isotropic .5 MPa experiment from Jacka [2]. Red dashed lines indicate MAP values. Parameters are shown in log-space where appropriate, with physical units given in brackets.

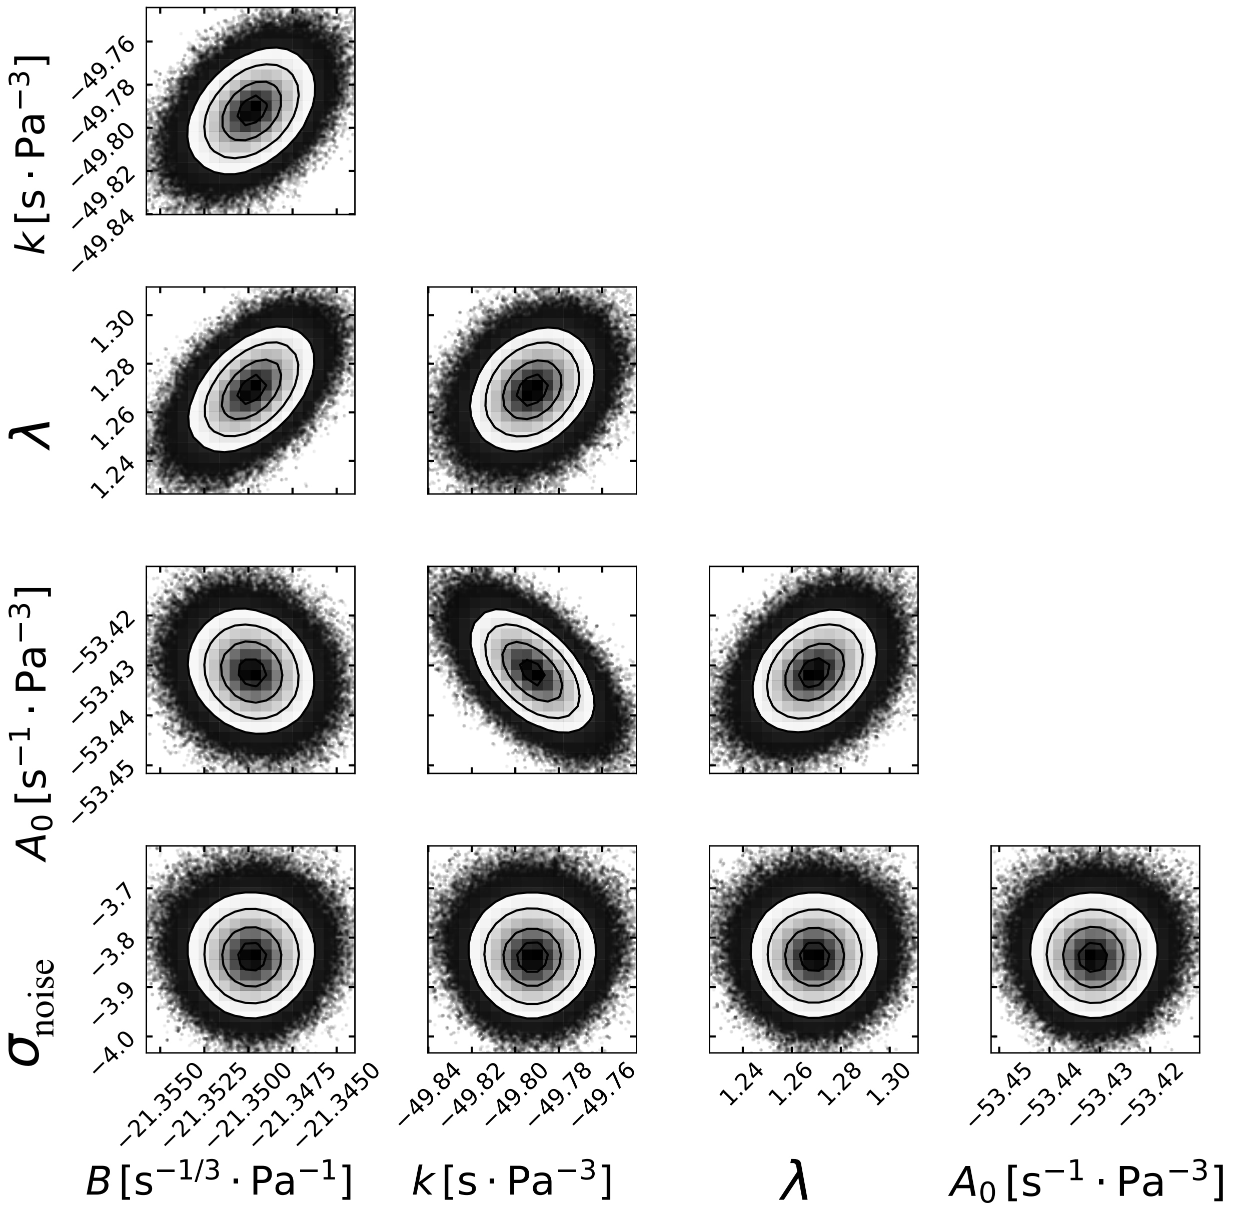


FIG. S25. Free parameters correlations from the MCMC fit for the isotropic .2 MPa experiment from Gao and Jacka [4]. Red dashed lines indicate MAP values. Parameters are shown in log-space where appropriate, with physical units given in brackets.

TABLE S2. Dataset-specific lognormal priors used for the MCMC fits for Jacka [2], Jacka and Maccagnan [3], Gao and Jacka [4]. Each parameter is defined in log-space with standard deviation $\sigma = 3.0$.

| **Gao & Jacka (1987), 0.2 MPa, 270 K** | |
|---|---|
| Parameter | Prior |
| $\log_{10} B$ | Lognormal($\mu = \log 1.0{\times}10^{-9}$, $\sigma = 3.0$) |
| $\log_{10} k$ | Lognormal($\mu = \log 1.0{\times}10^{-22}$, $\sigma = 3.0$) |
| $\log_{10} A_0$ | Lognormal($\mu = \log 1.0{\times}10^{-23}$, $\sigma = 3.0$) |
| $\log_{10} \lambda$ | Lognormal($\mu = \log 1.0{\times}10^{1}$, $\sigma = 3.0$) |
| $\log_{10} \sigma_{\text{noise}}$ | Lognormal($\mu = \log 1.0{\times}10^{-1}$, $\sigma = 3.0$) |
| $p$ | Fixed at $p = 3$ |
| **Jacka & Maccagnan (1984), 0.2 MPa, 264 K** | |
| $\log_{10} B$ | Lognormal($\mu = \log 1.0{\times}10^{-9}$, $\sigma = 3.0$) |
| $\log_{10} k$ | Lognormal($\mu = \log 1.0{\times}10^{-32}$, $\sigma = 3.0$) |
| $\log_{10} A_0$ | Lognormal($\mu = \log 1.0{\times}10^{-23}$, $\sigma = 3.0$) |
| $\log_{10} \lambda$ | Lognormal($\mu = \log 1.0{\times}10^{1}$, $\sigma = 3.0$) |
| $\log_{10} \sigma_{\text{noise}}$ | Lognormal($\mu = \log 1.0{\times}10^{-2}$, $\sigma = 3.0$) |
| $p$ | Fixed at $p = 5$ |
| **Jacka (1984), 0.5 MPa, 270 K** | |
| $\log_{10} B$ | Lognormal($\mu = \log 1.0{\times}10^{-10}$, $\sigma = 3.0$) |
| $\log_{10} k$ | Lognormal($\mu = \log 1.0{\times}10^{-17}$, $\sigma = 3.0$) |
| $\log_{10} A_0$ | Lognormal($\mu = \log 1.0{\times}10^{-24}$, $\sigma = 3.0$) |
| $\log_{10} \lambda$ | Lognormal($\mu = \log 1.0{\times}10^{1}$, $\sigma = 3.0$) |
| $\log_{10} \sigma_{\text{noise}}$ | Lognormal($\mu = \log 1.0{\times}10^{-2}$, $\sigma = 3.0$) |
| $p$ | Fixed at $p = 2$ |

TABLE S3. Posterior MAP estimates and diagnostics for all four Treverrow *et al.* [1] MCMC fits (uniform priors; mean acceptance rates 41–46%).

| Parameter | MAP | 95% CI | $\hat{R}$ | ESS |
|---|---|---|---|---|
| **Isotropic 0.2 MPa** | | | | |
| $B$ | $7.77\times10^{-10}$ | $[7.67\times10^{-10}, 7.86\times10^{-10}]$ | 1.000 | 41192 |
| $k$ | $6.94\times10^{-22}$ | $[6.54\times10^{-22}, 7.34\times10^{-22}]$ | 1.000 | 40514 |
| $A_0$ | $1.08\times10^{-23}$ | $[1.06\times10^{-23}, 1.10\times10^{-23}]$ | 1.000 | 40806 |
| $\lambda$ | 6.97 | [6.38, 7.62] | 1.000 | 40084 |
| $\sigma_{\text{noise}}$ | $4.47\times10^{-2}$ | $[4.01\times10^{-2}, 5.37\times10^{-2}]$ | 1.000 | 41262 |
| **Anisotropic 0.2 MPa** | | | | |
| $B$ | $1.32\times10^{-9}$ | $[1.30\times10^{-9}, 1.33\times10^{-9}]$ | 1.000 | 17916 |
| $k$ | $4.37\times10^{-22}$ | $[3.76\times10^{-22}, 5.10\times10^{-22}]$ | 1.000 | 18292 |
| $A_0$ | $7.76\times10^{-24}$ | $[7.62\times10^{-24}, 7.90\times10^{-24}]$ | 1.000 | 19166 |
| $\lambda$ | $9.31\times10^{-1}$ | $[8.21\times10^{-1}, 1.06]$ | 1.000 | 18352 |
| $\sigma_{\text{noise}}$ | $3.27\times10^{-2}$ | $[2.88\times10^{-2}, 4.07\times10^{-2}]$ | 1.000 | 20078 |
| **Isotropic 0.4 MPa** | | | | |
| $B$ | $8.68\times10^{-10}$ | $[8.54\times10^{-10}, 8.81\times10^{-10}]$ | 1.000 | 44449 |
| $k$ | $4.78\times10^{-22}$ | $[4.36\times10^{-22}, 5.25\times10^{-22}]$ | 1.000 | 44721 |
| $A_0$ | $1.21\times10^{-23}$ | $[1.16\times10^{-23}, 1.26\times10^{-23}]$ | 1.000 | 43728 |
| $\lambda$ | $3.43\times10^{1}$ | $[2.77\times10^{1}, 4.35\times10^{1}]$ | 1.000 | 45558 |
| $\sigma_{\text{noise}}$ | $1.04\times10^{-1}$ | $[9.29\times10^{-2}, 1.23\times10^{-1}]$ | 1.000 | 44021 |
| **Anisotropic 0.4 MPa** | | | | |
| $B$ | $1.78\times10^{-9}$ | $[1.74\times10^{-9}, 1.81\times10^{-9}]$ | 1.000 | 48725 |
| $k$ | $1.40\times10^{-21}$ | $[1.15\times10^{-21}, 1.76\times10^{-21}]$ | 1.000 | 48726 |
| $A_0$ | $9.04\times10^{-24}$ | $[8.79\times10^{-24}, 9.29\times10^{-24}]$ | 1.000 | 47672 |
| $\lambda$ | 7.79 | [5.17, 13.1] | 1.000 | 49030 |
| $\sigma_{\text{noise}}$ | $8.45\times10^{-2}$ | $[7.51\times10^{-2}, 1.02\times10^{-1}]$ | 1.000 | 48464 |

† One outlier walker was detected and filtered in the anisotropic 0.4 MPa chain.

TABLE S4. Posterior MAP estimates and diagnostics for three additional MCMC fits (uniform priors; acceptance rates 43–46%).

| **Gao & Jacka (1987), 0.2 MPa, 270 K** | | | | |
|---|---|---|---|---|
| **Parameter** | **MAP** | **95% CI** | $\hat{R}$ | **ESS** |
| $B$ | $5.344{\times}10^{-10}$ | $[5.327{\times}10^{-10}, 5.362{\times}10^{-10}]$ | 1.030 | 1148 |
| $k$ | $2.372{\times}10^{-22}$ | $[2.311{\times}10^{-22}, 2.438{\times}10^{-22}]$ | 1.030 | 1112 |
| $A_0$ | $6.241{\times}10^{-24}$ | $[6.168{\times}10^{-24}, 6.312{\times}10^{-24}]$ | 1.030 | 1111 |
| $\lambda$ | 3.561 | [3.473, 3.646] | 1.030 | 1166 |
| $\sigma_{\text{noise}}$ | $2.121{\times}10^{-2}$ | $[1.93{\times}10^{-2}, 2.445{\times}10^{-2}]$ | 1.030 | 1106 |
| **Jacka & Maccagnan (1984), 0.2 MPa, 264 K** | | | | |
| $B$ | $4.639{\times}10^{-9}$ | $[4.568{\times}10^{-9}, 4.708{\times}10^{-9}]$ | 1.000 | 46344 |
| $k$ | $1.248{\times}10^{-32}$ | $[1.001{\times}10^{-32}, 1.573{\times}10^{-32}]$ | 1.000 | 46187 |
| $A_0$ | $1.202{\times}10^{-23}$ | $[1.105{\times}10^{-23}, 1.313{\times}10^{-23}]$ | 1.000 | 46103 |
| $\lambda$ | $1.199{\times}10^{1}$ | [8.766, 17.65] | 1.000 | 47873 |
| $\sigma_{\text{noise}}$ | $1.516{\times}10^{-1}$ | $[1.332{\times}10^{-1}, 1.963{\times}10^{-1}]$ | 1.000 | 45229 |
| **Jacka (1984), 0.5 MPa, 270 K** | | | | |
| $B$ | $1.031{\times}10^{-10}$ | $[1.024{\times}10^{-10}, 1.038{\times}10^{-10}]$ | 1.000 | 40237 |
| $k$ | $4.649{\times}10^{-17}$ | $[4.555{\times}10^{-17}, 4.738{\times}10^{-17}]$ | 1.000 | 41501 |
| $A_0$ | $2.990{\times}10^{-24}$ | $[2.968{\times}10^{-24}, 3.014{\times}10^{-24}]$ | 1.000 | 40912 |
| $\lambda$ | 9.024 | [8.713, 9.327] | 1.000 | 40984 |
| $\sigma_{\text{noise}}$ | $1.621{\times}10^{-2}$ | $[1.475{\times}10^{-2}, 1.868{\times}10^{-2}]$ | 1.000 | 40537 |

† One outlier walker was filtered in the Gao & Jacka (1987) chain; two were filtered in the Jacka (1984), 0.5 MPa chain.
